# Supplementary material for: A Comprehensive Survey of Artificial Intelligence Techniques for Talent Analytics
Source: arXiv:2307.03195 source file (2025-05-26)
Supplement: Supplementary file 1 [file Appendix.pdf]

## APPENDIX A

### SYSTEMATIC RESOURCES FOR TALENT ANALYTICS

To help the readers learn more effectively, we highlight the systematic resources provided in this survey as follows,

- Table S1 and S2 summarizes the data for talent analytics.
- Table S3 summarizes recent AI-based talent analytics efforts in the talent management scenario.
- Table S4 summarizes recent AI-based talent analytics efforts in the organization management scenario.
- Table S5 summarizes recent AI-based talent analytics efforts in the labor market analysis scenario.

## APPENDIX B

### DATA PROCESSING FOR TALENT ANALYTICS

In Section 2, we have introduced the major categories of data involved in talent analytics. In the Appendix, we provide additional details on data collection, data preprocessing, data cleaning and debiasing techniques, as well as the limitations of the current datasets and processing methods.

#### B.1 Data Collection

The source of recruitment data can be categorized into two types: internal data and external data. Correspondingly, data collection methodologies align with these source categories.

**Internal Data.** The Current business environment is typically dependent on data systems [306]. Internal data are collected from the internal enterprise management systems, which are known as enterprise resource planning (ERP) system [307], customer relationship management (CRM) system [308], and applicant tracking system (ATS) system [309]. ERP systems are comprehensive business management tools that integrate various functions such as finance, sales, materials management, HR, production planning, and supply chain. CRM systems facilitate customer interaction and communication, encompassing customer information management, sales opportunities, and customer service. An ATS is computer software that human resource departments use to process the overwhelming number of applications they receive for job openings. These systems orderly store recruitment, employee, and organizational data, facilitating efficient collection and processing.

**External Data.** As online services rapidly evolve, a growing number of individuals are turning to social media and job search websites to exchange job-related information and explore employment opportunities. These interactive platforms host a vast array of talent information due to their extensive user base. Additionally, third-party business investigation platforms provide detailed insights into companies and the relationships of their board members. Data acquisition methods on these platforms vary. Third-party data collection websites typically aggregate data from their participating members. Meanwhile, web crawlers [310] can extract rich information from website pages, provided legal and regulatory compliance is ensured. Moreover, many job search websites retain substantial amounts of user data that isn't publicly disclosed. Typically, this data can be utilized for scientific research purposes following encryption and other privacy safeguards.

#### B.2 Data Preprocessing

After collecting a large amount of recruitment data, it is essential to preprocess the data for downstream applications, especially removing noisy, redundant, irrelevant, and potentially toxic data. In this part, we review the detailed data preprocessing strategies to improve the quality of the collected data according to various data types.

**Structured Data.** Structured data, in simple terms, is a database such as ERP system [313], that has a standardized format for efficient access by software and humans alike. Besides, the information of employees and companies is orderly collected into the database. On some data collection websites, a lot of user information is also strictly stored through databases, such as records of interactions between users and the platform, including clicking and browsing. Since these data have been stored in a standardized format, filtering and integration of corresponding data can generally be achieved by connecting different tables and setting data filtering conditions on the tables [314].

**Semi-Structured Data.** Semi-structured data, or partially structured data, diverges from the conventional tabular format characteristic of relational databases or other tabular data forms [315]. Instead, it incorporates tags and meta-data to delineate semantic elements and establish hierarchical relationships among records and fields. This type of data is prevalent in the labor market [316], encompassing employee resumes [317], individual interviews [318], job postings [319], and web pages [320]. Due to the absence of standardized formats and the diversity of semi-structured data types, it necessitates thorough exploration of commonalities, extraction of multidimensional information, and comprehensive filtering to transform it into structured data. For example, *Sun et al.* collected job postings from an online recruitment website [48]. On this website, each job opening is displayed in HTML, which contains information of salary range, company, location, time, and job description text. They parsed the HTML and obtained structured job posting information.

**Unstructured Data.** Unstructured data [321] refers to information that does not conform to the conventional row-column structure found in traditional databases. Within the labor market context, data primarily manifests as text, comprising a blend of structured and unstructured fields. Structured fields denote specific categories like job titles (e.g., occupation), location, etc., while unstructured fields provide a broader description of vacancy content. Approximately 80% of data held by firms today is unstructured [322], expanding at a rate fifteen times faster than structured data. While some approaches skip the processing of natural text, opting instead for direct classification tasks on such text, as observed in the classification of web job vacancies [323], others require extraction and subsequent processing of information from unstructured data into structured data. For instance, extracting skill information from job descriptions [86] involves the identification of skill words through regular expression matching. These identified words are then subjected to expert evaluation for further refinement, resulting in a set of relevant skill words for each job description. Subsequent statistical analysis across all jobs yields a comprehensive frequency distribution of skill words as

TABLE S1: The table of collected papers related to talent analytics-related data.

| Categories             | Data                   | Reference                       |
|------------------------|------------------------|---------------------------------|
| Internal: Recruitment  | Resume                 | [34, 35, 37, 38, 169, 179]      |
|                        | Job Posting            | [4, 10, 24, 36, 47, 48, 244]    |
|                        | Interview-related      | [31, 49, 50, 51, 52, 142]       |
| Internal: Employee     | Employee Profiles      | [6, 25, 55, 56, 57, 65, 169]    |
|                        | Training Records       | [58, 59, 60, 61, 284, 311, 312] |
| Internal: Organization | Reporting Lines        | [25, 26]                        |
|                        | In-firm Social Network | [55, 63, 64, 65]                |
| External               | Social Media           | [66, 67]                        |
|                        | Job Search Websites    | [27, 28, 68, 69, 70][71]        |

TABLE S2: The table of collected talent analytics-related open datasets.

| Categories           | Dataset                           | Link                                                                                                                                                                    | Note                                                                                                     |
|----------------------|-----------------------------------|-------------------------------------------------------------------------------------------------------------------------------------------------------------------------|----------------------------------------------------------------------------------------------------------|
| Internal:Recruitment | Kaggle-Entity_Recognition_Resumes | <a href="https://www.kaggle.com/datasets/dataturks/resume-entities-for-ner">https://www.kaggle.com/datasets/dataturks/resume-entities-for-ner</a>                       | 220 resumes; 10 categories; Resume Understanding                                                         |
|                      | LinkedIn-Job-Scraper              | <a href="https://www.kaggle.com/datasets/arshkon/linkedin-job-postings/data">https://www.kaggle.com/datasets/arshkon/linkedin-job-postings/data</a>                     | 33,000+ job postings; 27 valuable attributes including the title, job description, salary, location, etc |
|                      | Job Dataset                       | <a href="https://www.kaggle.com/datasets/ravindrasinghrana/job-description-dataset">https://www.kaggle.com/datasets/ravindrasinghrana/job-description-dataset</a>       | synthetic job postings; 23 attributes including job title, job salary, job skill, etc                    |
|                      | Linkedin Jobs & Skills (2024)     | <a href="https://www.kaggle.com/datasets/asaniczka/1-3m-linkedin-jobs-and-skills-2024">https://www.kaggle.com/datasets/asaniczka/1-3m-linkedin-jobs-and-skills-2024</a> | 12,96,381 job postings; skills mapping, job recommendation systems                                       |
| Internal:Employee    | HR Analytics                      | <a href="https://www.kaggle.com/datasets/colara/hr-analytics">https://www.kaggle.com/datasets/colara/hr-analytics</a>                                                   | 14999 employees; 10 attributes,including satisfaction_level, salary, etc; turnover prediction            |
|                      | Human Resources Data Set          | <a href="https://www.kaggle.com/datasets/rhuebner/human-resources-data-set/data">https://www.kaggle.com/datasets/rhuebner/human-resources-data-set/data</a>             | 311 records; 36 attributes, including name, salary, etc                                                  |

structured data, facilitating downstream tasks such as skill demand forecasting.

### B.3 Data Cleaning and Debias

After initial data preprocessing, standard structured data is obtained. However, given the potential for noise introduced during the data acquisition process, coupled with non-uniform acquisition methods, the provided data may not be of high quality. Therefore, a cleanup and debiasing of the data becomes imperative. In this part, we first introduce several data quality issues commonly seen in AI-driven talent analytics. Subsequently, several clean and debias methods are introduced to solve these issues.

**Data Quality Issues.** There are various data quality issues: missing data, duplicated data, extraneous data, and inconsistent data [324]. These issues will introduce biases into analyses and lead to inaccurate conclusions. We introduce these issues as follows:

- **Missing Data:** Missing data occurs when essential data is absent from a dataset, which can result from factors like data corruption, or failure to capture specific information. Within the talent market, missing values often stem from inconsistent information sources. For instance, job postings that should contain recruitment requirements and descriptions may be missing key

fields [325]. Resumes also frequently omit crucial information such as email addresses and physical addresses [326].

- **Duplicated Data:** Duplicated data refers to the presence of identical or nearly identical records within a dataset, which can arise from data entry errors, erroneous dataset merging, or technical malfunctions. Duplicated data can distort statistical analyses and exaggerate the significance of certain data points. In the talent market, this issue can arise due to data sources providing overly homogeneous information. Repetitive job postings may be erroneously interpreted as multiple postings for the same position in certain analysis and prediction scenarios [48].
- **Extraneous Data:** Extraneous data comprises irrelevant or unnecessary information within a dataset, often included mistakenly due to human errors or incorrect data integration processes. Such data can complicate analyses, waste computational resources, and yield inaccurate results. This data often requires further filtering to retain only relevant fields and eliminate irrelevant information, as noted in [327, 328]. Redundancies in job offers can hinder the accuracy of downstream classification tasks [328].
- **Inconsistent Data:** Inconsistent data encompasses con-

flicting or contradictory information within a dataset, stemming from sources like data entry errors, incompatible formats, or changes in data collection methods over time [325, 327, 329]. Such inconsistencies impede meaningful insights and necessitate thorough validation and cleansing to ensure data integrity and accuracy. Common inconsistencies include misspellings and variations in job titles, which require resolution to maintain consistency across professional documents [327, 329]. Besides, erroneous labeling of job postings as job titles is also a common problem [329].

**Cleaning and Debias Methods.** Data cleaning and debiasing is an iterative process tailored to the requirements and semantics of specific analysis tasks [351]. This process consists of transforming raw data into consistent data that can be analyzed. Herein, we delineate several frequently employed methodologies in talent analytics for data cleaning and debiasing.

- **Data Selection:** Data selection involves the meticulous identification and extraction of pertinent data subsets from a broader dataset, guided by specific criteria or requisites [352]. This approach serves to streamline the data analysis process by honing in on the most relevant information, thereby mitigating noise and extraneous data. For instance, *Zhang et al.* [10] opted to discard company-position pairs with a monthly averaged talent demand of less than 2, considering scenarios where certain companies may not extensively recruit for particular research positions, resulting in consistently low demand. *Shao et al.* conducted data cleaning by eliminating job posts and resumes with incomplete attributes [326]. *Balaji et al.* focused on extracting useful fields from job titles to curate the most pertinent and distinctive set of work activities corresponding to selected company job titles [327].
- **Data Filtering:** Data filtering encompasses the systematic elimination or exclusion of undesirable or extraneous data from a dataset, thereby diminishing noise and refining its quality. In typical text cleaning tasks, the compilation of a stop word list proves indispensable for sieving out irrelevant information [353]. Moreover, the adoption of regular expressions to delineate fields and detect anomalies is widely embraced in personalized resume-job matching systems [353] and job search engines [354].
- **Data Clustering:** Data clustering involves grouping similar data points together based on certain characteristics or features. *Wakchaure et al.* [355] leverages the Levenshtein edit distance, a metric gauging string similarity, to designate matches exceeding 0.85 as identical individuals. *Gaikwad et al.* [329] employs Levenshtein edit distance for duplicate detection within XML documents. *Sun et al.* [48] utilize text embedding and measure edit distance to approximate similar job descriptions. *Zhang et al.* [10] employ a classification approach to categorize original job titles into 16 distinct categories, thereby mitigating noise and standardizing job titles.
- **Data Synthesis:** Data synthesis encompasses the generation of fresh data points to augment extant datasets,

proving instrumental in addressing gaps or amplifying the efficacy of analysis and model functionalities [325]. For instance, *Magron et al.* [356] devised synthetic job postings to refine skill alignment, while *Skondras et al.* [357] utilized Large Language Models to craft synthetic resume data, thereby bolstering job description classification.

- **Data Normalization:** Data normalization is a crucial procedure aimed at standardizing the scale or distribution of data values within a dataset, thereby facilitating precise comparisons and analyses while ensuring uniformity across variables. It finds widespread application in various domains, particularly in time series forecasting. For instance, *Liu et al.* conducted normalization operations, which involve subtracting the minimum value of each node and dividing it by the difference between the maximum and minimum values of the node [231]. Similarly, *Zhang et al.* normalized the number of job transitions along the company axis to achieve consistency [230].

## B.4 Limitations

Existing data and processing methods in the field of talent analytics continue to face many limitations and challenges, which constrain the development of AI-based approaches. We summarize these issues as follows.

- **Lack of benchmark datasets:** Most current research in talent analytics heavily depends on proprietary data related to job applicants, employees, and organizations. As previously mentioned, internal data includes sensitive private information, such as the profiles of both job seekers and employees. The sensitive nature of this data often prevents it from being publicly accessible, severely restricting the development of publicly available benchmark datasets. This limitation impedes the standardization of problem definitions and comparative analyses of methodologies, thus slowing down technological advancements in the field. While some job-related data has been made open-source, it remains limited in scale and temporal coverage. Moreover, while existing methods utilize these data, they lack sufficient data analysis to provide researchers with meaningful insights. Consequently, there is an urgent need to create comprehensive open-source benchmark datasets for pivotal tasks within this field. We present several open datasets, as shown in the Appendix, primarily related to resume parsing and employee turnover prediction. These datasets can help researchers in developing standardized datasets for uniform comparisons. Additionally, the data anonymization and de-identification methods require more extensive consideration to facilitate the construction of more open-source datasets for various scenarios. Indeed, such technologies have been widely researched in the medical field [358, 359, 360]. In the context of talent analytics, *Jensen et al.* recently enhanced de-identification performance by integrating NER techniques with BERT for job postings [361]. However, current techniques often compromise data utility, especially for fairness and diversity analysis. Developing more advanced methods will allow the

TABLE S3: The table of collected papers related to talent management.

| Task                              | Method                                      | Data                                                            | Reference                                  |
|-----------------------------------|---------------------------------------------|-----------------------------------------------------------------|--------------------------------------------|
| <b>Talent Recruitment</b>         |                                             |                                                                 |                                            |
| Job Posting Generation            | RNN                                         | Job posting                                                     | [73, 80]                                   |
| Job Posting Generation            | LLMs                                        | Job posting                                                     | [81, 82]                                   |
| Resume Understanding              | Rule-base method                            | Resume                                                          | [89]                                       |
| Resume Understanding              | HMM                                         | Resume                                                          | [90]                                       |
| Resume Understanding              | SVM                                         | Resume                                                          | [90, 330]                                  |
| Resume Understanding              | CRF                                         | Resume                                                          | [32, 331]                                  |
| Resume Understanding              | LSTM,CNN                                    | Resume                                                          | [91]                                       |
| Resume Understanding              | LSTM,CRF                                    | Resume                                                          | [92, 92, 94, 332]                          |
| Resume Understanding              | RoBERTa,GCN                                 | Resume                                                          | [95]                                       |
| Resume Understanding              | Multimodal pre-trained model                | Resume                                                          | [33, 96]                                   |
| Talent Searching                  | Keywords matching                           | Query, Resume                                                   | [75]                                       |
| Talent Searching                  | Keywords matching, knowledge graph          | Query, Resume                                                   | [99]                                       |
| Talent Searching                  | Traditional classifiers                     | Query, Resume                                                   | [100, 101]                                 |
| Talent Searching                  | Topic model, multi-armed bandit algorithm   | Query, Resume                                                   | [102]                                      |
| Talent Searching                  | Learning-to-rank algorithm                  | Query, Resume                                                   | [74, 88]                                   |
| Talent Searching                  | DNN, learning-to-rank algorithm             | Query, Resume                                                   | [103, 104]                                 |
| Person-Job Fitting                | Latent variable model                       | Job posting, resume                                             | [108]                                      |
| Person-Job Fitting                | CNN                                         | Job posting, resume                                             | [36, 109, 120, 333]                        |
| Person-Job Fitting                | RNN                                         | Job posting, resume                                             | [4, 41, 334]                               |
| Person-Job Fitting                | CNN, RNN                                    | Job posting, resume                                             | [24, 111, 119]                             |
| Person-Job Fitting                | BERT                                        | Job posting, resume                                             | [112, 113, 114, 326], [115, 116, 335, 336] |
| Person-Job Fitting                | GNN, BERT                                   | Job posting, resume                                             | [5, 110, 117, 128, 337]                    |
| Person-Job Fitting                | Attention mechanism                         | Job posting, resume                                             | [107, 121, 122, 131]                       |
| Person-Job Fitting                | Reinforcement learning                      | Job posting, resume                                             | [123]                                      |
| Person-Job Fitting                | Federated learning                          | Job posting, resume                                             | [105]                                      |
| Person-Job Fitting                | LLMs                                        | Job posting, resume                                             | [118, 135, 136, 338, 339]                  |
| Person-Job Fitting                | Ranking                                     | Job posting, resume, social media                               | [125, 340]                                 |
| Person-Job Fitting                | K-means                                     | Social media                                                    | [341]                                      |
| Person-Job Fitting                | Traditional classifiers                     | Social media                                                    | [342]                                      |
| Person-Job Fitting                | Gamma-Poisson model                         | User behavior                                                   | [343]                                      |
| <b>Talent Assessment</b>          |                                             |                                                                 |                                            |
| Interview Question Recommendation | Topic model                                 | Job posting, resume, assessment report                          | [31, 49]                                   |
| Interview Question Recommendation | Knowledge graph                             | Job posting, resume, search engine log                          | [42]                                       |
| Interview Question Recommendation | Knowledge graph, integer linear programming | Question bank                                                   | [137]                                      |
| Interview Question Recommendation | BERT                                        | Job posting                                                     | [77]                                       |
| Interview Question Recommendation | GCN                                         | KSC, search engine log                                          | [43]                                       |
| Assessment Scoring                | Regression models                           | Interview videos                                                | [141, 144, 344]                            |
| Assessment Scoring                | Doc2Vec                                     | Interview videos                                                | [50, 142]                                  |
| Assessment Scoring                | GNN                                         | Interview records                                               | [52]                                       |
| Assessment Scoring                | Attention mechanism                         | Interview videos                                                | [51, 143, 345]                             |
| Assessment Scoring                | Transformer                                 | Interview videos                                                | [145, 346]                                 |
| Assessment Scoring                | Adversarial learning                        | Interview videos                                                | [146]                                      |
| Assessment Scoring                | traditional classifiers                     | Employee profiles                                               | [60, 61, 312]                              |
| <b>Career Development</b>         |                                             |                                                                 |                                            |
| Course Recommendation             | Collaborative filtering                     | Trainees' profiles                                              | [58, 284]                                  |
| Course Recommendation             | Markov decision process                     | Learning records                                                | [59]                                       |
| Course Recommendation             | Neural Network                              | Learning records                                                | [151]                                      |
| Course Recommendation             | Reinforcement Learning                      | Learning records                                                | [152]                                      |
| Course Recommendation             | KG-based Transformer                        | Learning records, Knowledge Graph                               | [153]                                      |
| Promotion Prediction              | Traditional classifiers                     | Social network                                                  | [158]                                      |
| Promotion Prediction              | Traditional classifiers                     | Personal profile, job posting log                               | [79]                                       |
| Promotion Prediction              | Multiple classification                     | Employee's Detail Record                                        | [159]                                      |
| Promotion Prediction              | Survival analysis                           | Personal profile, career paths                                  | [6]                                        |
| Turnover Prediction               | Traditional classifiers                     | HR dataset                                                      | [164, 165, 347]                            |
| Turnover Prediction               | GNN, RNN                                    | profile, turnover records                                       | [56]                                       |
| Turnover Prediction               | neural network                              | profile, turnover records                                       | [65]                                       |
| Turnover Prediction               | Traditional classifiers                     | HR Information Systems                                          | [348]                                      |
| Turnover Prediction               | GNN, RNN, survival analysis                 | job description, organizational tree, profile, turnover records | [57]                                       |
| Job Satisfaction                  | Traditional classifiers                     | Personal profile, job profile                                   | [171]                                      |
| Job Satisfaction                  | Traditional classifiers                     | Social media                                                    | [172]                                      |
| Career Mobility Prediction        | RNN                                         | Career paths                                                    | [177, 180]                                 |
| Career Mobility Prediction        | Attention mechanism                         | Career paths, employee profile                                  | [38]                                       |
| Career Mobility Prediction        | Transformer                                 | Career paths, employee profile                                  | [178]                                      |
| Career Mobility Prediction        | Collaborative filtering                     | Career paths, employee profile                                  | [179]                                      |
| Career Mobility Prediction        | GNN                                         | Career paths, employee profile                                  | [169]                                      |
| Career Mobility Prediction        | Representation learning                     | Career paths, employee profile                                  | [181, 182]                                 |
| Career Mobility Prediction        | Reinforcement learning                      | Career paths, employee profile                                  | [183, 349, 350]                            |

Traditional classifiers represent one or multiple traditional classifiers, including SVM, Logistic regression, GBDT, XGBoost, Decision tree, Adaboost, KNN and so on.

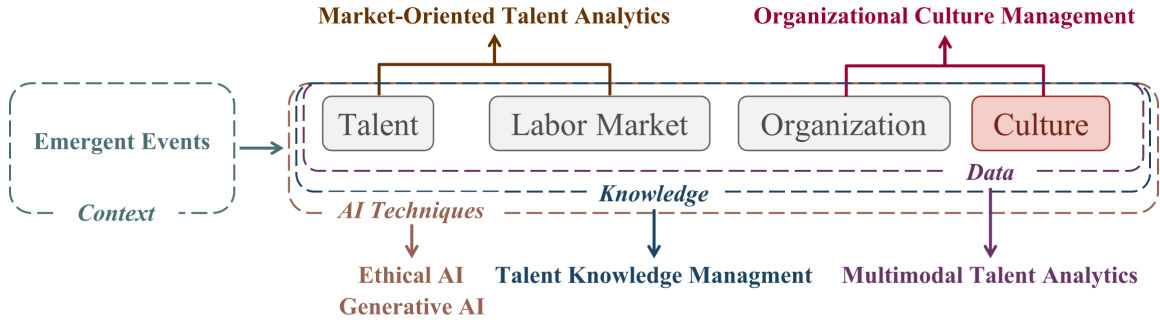

Fig. S1: The potential research directions in talent analytics.

creation of comprehensive, privacy-preserving datasets that retain key demographic variables, supporting both benchmarking and fairness research in talent analytics.

- **Diversity deficiencies in datasets:** The datasets commonly used in AI-based talent analytics often lack adequate consideration of diverse populations, especially underrepresented minorities. This deficiency hampers efforts to evaluate and ensure algorithmic fairness. Models developed from such datasets may exhibit biases, leading to inequitable outcomes among various demographic groups. Furthermore, the absence of publicly available gender and racial data restricts the ability to conduct comprehensive fairness evaluations, making it difficult to detect and mitigate biases effectively. Therefore, it is essential to integrate more diverse datasets to promote fairness and enhance the overall performance of AI algorithms in talent analytics.
- **Challenges with subjective data:** In many talent analytics scenarios, such as employee promotion decisions, outcomes are frequently based on the subjective judgment of supervisors. This practice can introduce inherent biases and noise into the real datasets collected from these decisions. Traditional data preprocessing techniques often fail to detect and address these anomalies effectively. Therefore, there is a pressing need for specialized noise detection algorithms or the development of robust AI-based talent analytics models that can handle such irregularities. These approaches are essential to ensure the accuracy and fairness of the analytics outcomes.

## APPENDIX C PROSPECTS

In this appendix, we provided a broader and specific recent efforts in AI-based talent analytics in human resource management from three different aspects: talent management, organization management, and labor market analytics, which can provide a more detailed explanation and discussion for the prospects section in the main text.

### C.1 Multimodal Talent Analytics

Information about a phenomenon or a process in talent analytics-related scenarios usually comes in different modalities. For instance, we can obtain communication and

project collaboration networks in employee collaboration analysis. Indeed, mining the multimodal data in talent analytics can help us enhance the effectiveness of different applications. For example, *Hemamou et al.* collected the multimodal data in the job interview process, including text, audio, and video, and proposed a hierarchical attention model to achieve the best performance in predicting the hirability of the candidates [51]. Moreover, the utilization of multimodal data to train AI models, rather than solely relying on traditional interviews, offers a more comprehensive understanding of the participants' personality test results [279]. Recently, multimodal learning has been used to achieve multimodal data representation, translation, alignment, fusion, and co-learning in various domains, such as commercial, social, biomedical [280, 281]. We can foresee that more multimodal learning methods will gradually be extensively used in talent analytics.

### C.2 Talent Knowledge Management

Though AI-based approaches have achieved great success in acquiring talents and developing them, relatively few works explore managing those talents' knowledge with AI technologies, which is the primary driving force to the economics of ideas [282]. There is an urgent need for additional AI-based technologies that focus on talent knowledge creation, sharing, utilization, and management. Such efforts are crucial for maximizing the potential of human resources and enhancing organizational productivity. Indeed, we can leverage knowledge graph-related technologies [283] to construct the talent's knowledge base and achieve efficient knowledge management. Moreover, we can transform the scenarios in talent development, such as knowledge learning and collaboration, into different recommendation scenarios and utilize recommendation algorithms to solve these problems. Recently, *Wang et al.* developed a personalized online courses recommendation system based on the employees' current profiling [58, 284]. However, there is still a lack of an algorithm that can recommend heterogeneous knowledge. The existing algorithms are only from the individual perspective and have not been analyzed from the organizational aspect, such as the organizational knowledge diversity or competitiveness. Furthermore, although AI-based technologies have greatly improved the efficiency of knowledge management, the social and ethical implications (algorithmic discrimination, etc.) that they bring with them are also worthy of continued research [363].

TABLE S4: The table of collected papers related to organizational management.

| Task                                     | Method                                       | Data                                  | Reference  |
|------------------------------------------|----------------------------------------------|---------------------------------------|------------|
| <b>Organizational Network Analysis</b>   |                                              |                                       |            |
| Organizational Network Modeling          | Representation learning                      | Organizational network dataset        | [7]        |
| Organizational Network Modeling          | GCN, RNN                                     | Working related records               | [65]       |
| Organizational Network Modeling          | Community Search                             | Public data, in-firm data             | [362]      |
| High-potential Talent Identification     | GNN, LSTM                                    | Organizational network dataset        | [55]       |
| <b>Organizational Stability</b>          |                                              |                                       |            |
| Team formation                           | Heuristic algorithm                          | DBLP, IMDb                            | [196]      |
| Team formation                           | Greedy algorithm                             | DBLP                                  | [197]      |
| Team formation                           | Variational Bayes Network                    | DBLP                                  | [199]      |
| Team formation                           | Hybrid approach                              | Crowdsourcing data                    | [203]      |
| Team formation                           | Greedy algorithm                             | Freelancer dataset                    | [204]      |
| Team formation                           | Adaptive algorithm                           | Crowdsourcing data                    | [205]      |
| Team optimization                        | Graph kernel                                 | DBLP, Movie and NBA                   | [207, 208] |
| Team optimization                        | Deep learning                                | GitHub, DBLP                          | [211]      |
| Team optimization                        | Reinforcement learning                       | Movie, DBLP                           | [212]      |
| Person-Organization Fit                  | CNN, LSTM                                    | In-firm data                          | [25, 26]   |
| Person-Organization Fit                  | KNN                                          | Talent data                           | [215]      |
| <b>Organizational Incentive Analysis</b> |                                              |                                       |            |
| Job title benchmarking                   | Representation Learning                      | OPNs                                  | [187]      |
| Job title benchmarking                   | Semantic relatedness modeling                | CEDEFOP classify Online Job Vacancies | [218]      |
| Job title benchmarking                   | Graph learning                               | Working experiences and resume data   | [216]      |
| Job title benchmarking                   | BiLSTM, Unsupervised representation learning | A labeled job similarity dataset      | [217]      |
| Job title benchmarking                   | Transformer, RNN                             | Employee career paths in IT field     | [114]      |
| Job title benchmarking                   | Bert, Graph embedding                        | Resume data                           | [220]      |
| Job salary benchmarking                  | Matrix completion                            | Job posting                           | [46, 223]  |
| Job salary benchmarking                  | Matrix equation                              | Job post and review data              | [224]      |

### C.3 Market-oriented Talent Analytics

AI technology has been effectively applied in labor market analytics [229]. However, those approaches mainly focus on the perspective of global market analysis and have not explored how the changing environment of the labor market affects internal talent management or organization management. In fact, combining macro and micro data in talent analytics is a vital research direction [364]. With the recent accumulation of internal and external data, there exists an exceptional opportunity to implement market-oriented talent analytics. For instance, *Hang et al.* leveraged the job posting data to capture the potential popularity of employees in external markets specific to skills and further achieve more accurate employee turnover prediction based on the market trend [57]. Moreover, the rapid development of AI technologies provides an excellent technical foundation for this direction. We can utilize multi-task learning [365] to jointly learn both macro and micro talent analytics-related tasks. Heterogeneous graph learning [57, 366] can help us effectively model the correlation of macro and micro data.

Besides, we can use AI technologies to identify various types of talents in the market. Identifying high-potential employees has always been an important issue in enterprises. *Ye et al.* [55] proposed a neural network-based dynamic social profiling approach for quantitatively identifying high-potential talents. *Cheng et al.* [193] conducted a quasi field experiment study and found that AI outperforms humans in the identification of high-potential talents. In the labor market, accurate recruitment of digital talents is crucial for the digital transformation of enterprises. *Harrigan et al.* [285] found a specific relationship between enterprise talent investment and digitization by identifying digital

skills-related talents within the organizations. By collecting data on workers, *Goos et al.* [367] found that people in regular jobs had a harder time finding jobs in new factories compared to digital talents. *Babina et al.* [286] classified different categories of AI skill-related talents based on job postings on recruitment platforms and analyzed the impact of these talents on the development of the enterprise after entering the enterprise. *Kim et al.* [287] proposed a dynamic co-occurrence method, which dynamically calculates the AI relevance of various types of skills in the labor market, so as to identify AI talents more accurately. It can be seen that AI has a great impact on human resource management, especially in the current situation where enterprises are paying more and more attention to environmental protection and social responsibility, AI has a broad prospect in the identification of green talents and Environmental, Social and Governance (ESG)-related talents. AI and human resource management still need large-scale research in the future.

### C.4 Organizational Culture Management

In our survey, we reviewed recent advancements in AI techniques for talent analytics in HRM from three perspectives, including talent management, organization management, and labor market analysis. The culture of an organization plays a crucial role in sustaining its effectiveness and viability [288]. Generally, the culture mainly contains three aspects: Mission, Vision, and Values (MVs), which can help employees understand what is encouraged, discouraged, accepted, or rejected within an organization, and facilitate the organization to thrive with the shared purpose. Recent developments reveal that the availability of extensive datasets covering the entire lifecycle of talents and orga-

TABLE S5: The table of collected papers related to labor market analysis.

| Task                        | Method                                        | Data                 | Reference            |
|-----------------------------|-----------------------------------------------|----------------------|----------------------|
| <b>Talent Flow Analysis</b> |                                               |                      |                      |
| Flow prediction             | RNN                                           | OPNs                 | [267]                |
| Flow prediction             | Tensor Factorization                          | OPNs                 | [230]                |
| Flow prediction             | Latent variable model                         | OPNs                 | [229]                |
| Flow prediction             | GAT                                           | Questionnaires       | [231]                |
| Flow prediction             | Graph Clustering, HITS                        | OPNs                 | [184]                |
| Flow pattern analysis       | Learning algorithms                           | OPNs                 | [233]                |
| Flow pattern analysis       | Optimization algorithm                        | OPNs                 | [232]                |
| Flow pattern analysis       | PageRank                                      | OPNs                 | [234, 235]           |
| Flow pattern analysis       | Clustering model                              | OPNs                 | [236]                |
| Flow pattern analysis       | Clustering model, PageRank                    | OPNs                 | [269]                |
| <b>Job Analysis</b>         |                                               |                      |                      |
| Demand trend analysis       | Latent Semantic Indexing                      | Job postings         | [238]                |
| Demand trend analysis       | N-gram, SVM                                   | Job postings         | [237]                |
| Demand trend analysis       | Attentive neural network                      | Job postings         | [10]                 |
| Demand Trend analysis       | Dynamic Graph                                 | Job postings         | [239]                |
| Topic Trend analysis        | Latent variable model                         | Job postings         | [9]                  |
| Topic Trend analysis        | Bi-gram model                                 | Job postings         | [270]                |
| Topic Trend analysis        | Word2Vec, RNN                                 | Job postings         | [271]                |
| Topic Trend analysis        | NER                                           | Job postings         | [272]                |
| <b>Skill Analysis</b>       |                                               |                      |                      |
| Potential Skill Prediction  | language models,SVM                           | Job postings         | [240]                |
| Potential Skill Prediction  | Apriori algorithm                             | Job postings         | [241]                |
| Potential Skill Prediction  | FP-growth algorithm                           | Job postings         | [242]                |
| Potential Skill Prediction  | KNN algorithm                                 | Job postings         | [243]                |
| Potential Skill Prediction  | Tensor factorization                          | Job postings         | [244]                |
| Potential Skill Prediction  | Topic model                                   | Job postings         | [47]                 |
| Potential Skill Prediction  | GNN                                           | Job postings         | [245]                |
| Potential Skill Prediction  | SDCA logistic regression                      | Job postings         | [246]                |
| Potential Skill Prediction  | Bert                                          | Job postings         | [247]                |
| Skill demand forecasting    | Logistic Regression, Granger Causality        | Job postings         | [248]                |
| Skill demand forecasting    | Bert, Logistic Regression, Random forest, SVC | Job postings         | [249]                |
| Skill demand forecasting    | RNN                                           | Job postings         | [250]                |
| Skill demand forecasting    | LSTM, TimeGAN                                 | Job postings         | [251]                |
| Skill demand forecasting    | Hypernetwork, RNN                             | Job postings         | [252]                |
| Skill demand forecasting    | Pretraining Graph Autoencoder                 | Job postings         | [86]                 |
| Skill Valuation             | Hill climbing                                 | Dblp                 | [253]                |
| Skill Valuation             | Neural network                                | Job postings         | [48]                 |
| Skill Valuation             | Linear regression                             | Job postings         | [254]                |
| <b>Brand Analysis</b>       |                                               |                      |                      |
| Employer branding           | Topic Regression                              | Job reviews          | [27, 28]             |
| Employer branding           | ELM classifier                                | Company reviews      | [68]                 |
| Employer branding           | Markov switching model                        | News, Social media   | [67]                 |
| Employer branding           | Prototype representation                      | Corporate events     | [255]                |
| Employer branding           | Extreme learning machine                      | Job reviews          | [256]                |
| Employer branding           | Topic model                                   | Company descriptions | [257]                |
| CSR communication           | Topic model                                   | Social media         | [258, 259, 260, 261] |
| Employee sentiment analysis | Topic Model                                   | Company reviews      | [228]                |
| Employee sentiment analysis | Topic model                                   | Social media         | [66]                 |
| Employee sentiment analysis | Topic model                                   | Job reviews          | [262, 263]           |
| Employee sentiment analysis | TF-IDF, Bag of words, SVM                     | Job reviews          | [264, 265]           |
| Employee sentiment analysis | CNN, RNN                                      | Job reviews          | [266]                |

nizations offers opportunities to realize effective culture management. For example, the interconnection between culture and leadership is evident, with exceptional team leaders significantly shaping organizational culture [288]. Some researchers [289] discussed how ML techniques can be used to inform predictive and causal models of leadership effects. Accordingly, they further provided a step-by-step guide on designing studies that combine field experiments to establish causal relationships with maximal predictive power. Meanwhile, several studies analyze leadership styles with data mining algorithms, demonstrating that the differ-

ent leadership styles significantly influence leadership outcomes [290]. Moreover, some researchers try to utilize text mining to analyze the organizational culture. For instance, *Schmiedel et al.* leveraged the online company reviews data and topic model to explore the employees' perception of corporate culture [69]. *Li et al.* [368] applied a topic model to obtain firm-level measures of exposure and response related to emergent events for many U.S. firms. As a famous saying goes, "Culture eats strategy for breakfast", employing AI technologies in organizational culture management will become one of the most critical research directions in the

future, as it can help managers scientifically address cultural management.

## C.5 Ethical AI in Talent Analytics

Admittedly, AI technologies are increasingly employed in talent analytics, significantly enhancing management efficiency and accuracy. However, there are ongoing concerns about how to ensure that AI technologies adhere to well-defined ethical guidelines regarding fundamental values. Recently, some researchers have made efforts from two perspectives, i.e., fairness and explainability.

### C.5.1 Fairness

The importance of fairness in talent analytics cannot be overstated, given its profound impact on employee well-being and alignment with organizational values. Although AI technologies have achieved various successes in talent analytics, there is growing concern that such approaches may bring issues of unfairness to people and organizations, as evidenced by some recent reports [291, 369, 370]. For instance, Amazon scrapped its AI-based recruitment system due to its discriminatory outcomes against women [291].

Recent studies have delved into the fairness of AI technologies in talent management from different perspectives. For instance, *Qin et al.* [41] verified that when involving sensitive features, such as gender, age, etc., into the person-job fit model, the model without special design will easily learn the bias from the original data. Intuitively, we can solve this problem by removing sensitive features, also regarded as one of the pre-processing methods for imposing fairness [371]. However, a large amount of unstructured data already contains sensitive features, such as audio and video data in the interview process. The model can easily infer the potentially sensitive attributes of data, which may still cause the bias of AI algorithms [372]. In their study, *Pena et al.* examined multimodal systems to predict recruitable candidates using both image and structured data from resumes [35]. The authors first demonstrated that the deep learning model could reproduce the biases from the training data, even without the sensitive features. To address this, they integrated an adversarial regularizer to remove sensitive information from unstructured data and promote algorithmic fairness [373]. Similarly, *Yan et al.* both leveraged data balancing and adversarial learning to mitigate bias in the multimodal personality assessment [292]. Moreover, there exist several open-source tools, such as AIF360 [374], FairML [375], Themis-ML [376], that can facilitate systematic bias checks and embed fairness in the AI algorithms [377]. In addition, AI technologies can also help to reduce human bias in different talent management scenarios. For instance, AI technologies have been applied to detect the potentially problematic words in the job posting that lead to bias or even legal risks and further assist employers in writing inclusive job descriptions [378]. Consequently, ensuring the fairness of AI algorithms is becoming an increasingly significant area of research within the field of talent analytics.

### C.5.2 Explainability

Recently, there has been an increasing concern among employees and managers regarding the decisions made by

black-box AI algorithms. Questions arise regarding the basis of these decisions, understanding the factors behind algorithmic success or failure, and determining how to rectify any errors that occur. Therefore, the research interest in increasing the transparency of AI-based automated decision-making in talent management are re-emerging [379, 380]. For instance, *Qin et al.* proposed to leverage the attention mechanisms to explain the matching degree between the content of job postings and resumes [4]. *Zhang et al.* further introduced the hierarchical attention and collaborative attention mechanisms to increase the person-job fit model explainability both at the structured and unstructured information level [131]. *Upadhyay et al.* leveraged the knowledge graph and name entity recognition technologies to generate the understandable textual job recommendation explanation [381]. In [382], *Kaya et al.* focused on constructing an end-to-end system for explainable automatic job candidate screening from video resumes. The authors extracted the audio, face, and scene features and leveraged the decision trees to both predict whether the candidates will be invited to the interview and explain the decisions by using binarization with a threshold. *Liem et al.* further handled the job candidate screening problem from an interdisciplinary viewpoint of psychologists and machine learning scientists [383]. Moreover, *Juvitayapun et al.* utilized the tree-based model to calculate the importance of different features, enhancing the explainability of AI-based turnover prediction [166].

However, the current approaches only stay in the perspective of AI model design and fail to consider whether employees or managers can easily comprehend and grasp the explanatory conclusions provided by the model. Indeed, visual analytics is an inherent way to help people who are inexperienced in AI understand the data and model [384, 385]. Therefore, combining visual analysis and explainable AI and building an intelligent talent management system is a valuable research direction. Additionally, leveraging the extensive interaction data generated by users can facilitate iterative model improvements from various angles, including correcting errors in automated decision-making and enhancing the efficiency of visual information presentation.

## C.6 Generative AI in Talent Analytics

With technological advances, artificial intelligence has gradually developed a branch called generative AI, and the language in which AI interacts with humans has changed from “machine language” to “natural language” [293]. By employing suitable templates, many tasks can be addressed through generative AI. Specifically, the knowledge emergence facilitated by large-scale parameters enables generative AI to tackle a series of complex tasks [386]. The advent of generative LLMs has sparked widespread discussion and excitement in both academia and industry. First of all, LLMs have a strong generative ability, which enables them to easily understand various contexts and generate appropriate content according to the prompts. The following work is a good illustration of this aspect of the capabilities of LLMs: *Zinjad et al.* proposed a resume generation tool based on natural language understanding and information extraction



capabilities of LLMs, which allows users to generate tailored personalized resumes by providing simple personal information and job information [294]. *Ayoobi et al.* proposed a method for recognizing LLM-generated resumes in online recruitment platforms, which is beneficial in solving the challenge of identifying fake and LLM-created resumes that are difficult to identify [387]. *Magron et al.* constructed a job posting dataset for skill matching that contains more implicit skills, longer sentences, and is closer to data from real job platforms. They conduct skill-matching experiments using LLMs and show that the method performs well in real-world data evaluation [356]. Second, LLMs facilitate the innovation of traditional AI technologies. For example, in the context of recommender systems, LLMs utilize their high-quality representation of textual features and their extensive coverage of external knowledge to achieve high-quality recommendations [293]. *Wu et al.* revealed the capability of LLMs to mine graph information by proposing a meta-path prompt constructor to help LLMs understand the semantics of behavioral graphs, and the framework helps provide personalized job recommendations for job seekers [339]. *Du et al.* improved the traditional LLM-based job recommendation method and verified its effectiveness by mining the explicit and implicit features of users in an online recruitment platform, and aligning the unmatched low-quality and high-quality generated resumes via a generative adversarial network [136]. *Zheng et al.* guided the LLM-based generative job recommendation system based on a Supervised Fine-Tuning strategy, generate suitable job descriptions according to the resumes of job seekers, and provide individuals with a more personalized and comprehensive job-seeking experience [135]. *Abu-Rasheed et al.* developed a group chat method based on knowledge graphs to enhance the interpretability of students in conversations with chatbots in the course recommendation task [388].

Besides, in recent years, LLM-based agents are utilized to solve various tasks such as software development, social simulation, and policy simulation [295]. Research on intelligent simulation of management-related problems using digital technologies has also been emerging, such as the study of member autonomy in organizations using human-machine systems based on blockchain technology [296]; how humans can use AI assistants to work effectively with large language models [389]; and how autonomous agents can utilize the generic capabilities of the underlying model for reasoning, decision-making, and environment interaction [390]. Further, by integrating multiple LLM agents, model efficiency can be further improved and simulation effects can be optimized [297]. However, there is not much research on using agents based on large language models for simulating organizational behavior. We should use management theory to simulate the framework of an organization and the behavior of individuals within the organization, which can focus on the trust behavior of inter-organizational personnel in interpersonal interactions, i.e., the willingness to put one's self-interest at risk based on the positive expectations of others [298]. An LLM-based agent can be used to generate conversational data for studying the behaviors and capabilities of chat agents [391]. They query APIs that read and write to web pages, generate content that shapes human behavior, and run system commands as autonomous

agents [392]. We can also analyze LLMs' network formation behavior to examine whether the dynamics of multiple LLMs are similar to or different from human social dynamics [29]. In addition, LLM capabilities can be used to create professional agents with controlled, specialized, and interactive, professional-level capabilities to reshape professional services through evolving expertise [393]. There is an empirical result that shows the agent named QuantAgent is useful in financial research, as it has the capability to uncover viable financial signals and enhance the accuracy of financial forecasts [394]. In a study by *Yang et al.* [395], an agent-based model was developed to simulate the decision-making behavior and interactive behavior of enterprises and employees based on the HRM characteristics of growing enterprises. The study found that firms should pay extra attention to recruitment programs, changes in workers' pay gaps are influenced by industry growth and their own capabilities, and pay cap policies have a positive impact on the development of growth firms in the start-up stage. However, there is still a lack of research on Agent-based simulation of cooperative behaviors among employees with different competencies within an organization based on a large language model.

Finally, in the organization, managers use the knowledge inside and outside the organization to make procedural and non-procedural decisions to improve the scientificity and accuracy of decision making [396]. To further enhance decision-making efficiency, many organizational managers have introduced AI technologies for assistance. In particular, the recent rise of generative large language models (LLMs) offers new opportunities. These models demonstrate proactive interaction capabilities and can support not only individual decision-making and task execution but also organizational-level planning and scheduling [299]. For instance, *Zheng et al.* developed an LLM-based generative job recommendation system to provide individuals with a more personalized and comprehensive job seeking experience [135]. By imposing prompt-based organizational structures on LLM agents, *Guo et al.* [397] found that LLMs exhibit leadership and spontaneous cooperative behaviors in their organizations. In the decision-making process, it seems that human dominance has become weaker and AI's decision-making ability has become stronger, which makes it easier to correct the decision-making bias brought about by human intuition [398]. However, due to the algorithmic black box characteristics of generative AI, it is difficult for humans to intervene and predict the content generated by generative AI [399]. Therefore, in the decision-making process, generative AI may pose the risk of false information and misleading decisions [400, 401]. Therefore, in talent management, how to dialectically view AI and how to effectively use AI to manage and avoid risks is a key topic worthy of future research. However, the applications of existing LLMs in talent analysis also have limitations, such as the accuracy of generated information, interpretability, interaction forms, etc., which will affect the application of large models in business scenarios.

## C.7 The Impact of Emergent Events on Talent Analytics

Emergent events such as pandemics have had a huge impact on businesses and organizations, and there are many

management scenarios where we can apply AI methods to effectively deal with these dilemmas. In talent management, because of the pandemic, the daily tasks of the employees in many companies will change. In order to make the company adapt to this fluctuation and to mitigate the impact of these emergent events, we can predict the performance of the employees by using AI methods [300]. Additionally, the epidemic has taken a toll on numerous markets and industries, causing employees in companies to face high psychological stress, and some may even leave the organization. We can complete the simulation of employees' stress through AI technologies [402] and understand the factors that influence the employees' intention to leave the organization [403, 404]. From the perspective of an organization's leader, it is essential to understand the impact of the epidemic on customers so that an effective response can be taken. Therefore, completing sentiment analysis of customers using text is a very effective approach [301, 302]. Lastly, in the labor market, AI methods can effectively use large-scale data to provide researchers with research perspectives and technical support to study the impact of emergent events on the labor market [405, 406].

Besides organizational resilience, the forms of talent analytics are facing a transformation due to some emergent events. Because issues such as the need to limit social distances that arose during the epidemic triggered us to think about increasing human-computer interaction in the workplace scenario [407]. In the recruitment process, since global cooperation and telecommuting have become frequent, we can use AI technologies such as natural language processing technology to screen job applicants in global real-time big data [303], to reduce the risk of disease transmission in densely populated scenarios, the use of chatbots to communicate with onboarding employees during the onboarding process can avoid the contact of the employees and simplify the process of onboarding employees [304]. Once employees are onboarded, they can also be trained with the help of a robot [305]. Xu *et al.* found that applying AI-enhanced VR simulators to employee training can reduce human resource costs and increase employee satisfaction, thereby enhancing the competitiveness of the organization [408]. Finally, for managers of organizations, as the temporary workforce of organizations is increasing after the epidemic era, combining temporary workforce management with AI can reduce risks and costs and improve work efficiency and quality [409].

## REFERENCES

- [1] B. Sivathanu and R. Pillai, "Technology and talent analytics for talent management—a game changer for organizational performance," *International Journal of Organizational Analysis*, 2019.
- [2] A. Sharma and J. Bhatnagar, "Talent analytics: A strategic tool for talent management outcomes," *Indian Journal of Industrial Relations*, vol. 52, no. 3, pp. 515–527, 2017.
- [3] J. Kaur and A. A. Fink, "Trends and practices in talent analytics," *Society for Human Resource Management (SHRM)—Society for Industrial-Organizational Psychology (SIOP) Science of HR White Paper Series*, vol. 20, 2017.
- [4] C. Qin, H. Zhu, T. Xu, C. Zhu, L. Jiang, E. Chen, and H. Xiong, "Enhancing person-job fit for talent recruitment: An ability-aware neural network approach," in *The 41st international ACM SIGIR conference on research & development in information retrieval*, 2018, pp. 25–34.
- [5] K. Yao, J. Zhang, C. Qin, P. Wang, H. Zhu, and H. Xiong, "Knowledge enhanced person-job fit for talent recruitment," in *2022 IEEE 38th International Conference on Data Engineering (ICDE)*. IEEE, 2022, pp. 3467–3480.
- [6] H. Li, Y. Ge, H. Zhu, H. Xiong, and H. Zhao, "Prospecting the career development of talents: A survival analysis perspective," in *Proceedings of the 23rd ACM SIGKDD International Conference on Knowledge Discovery and Data Mining*, 2017, pp. 917–925.
- [7] Y. Ye, Z. Dong, H. Zhu, T. Xu, X. Song, R. Yu, and H. Xiong, "Mane: Organizational network embedding with multiplex attentive neural networks," *IEEE Transactions on Knowledge and Data Engineering*, 2022.
- [8] H. Wi, S. Oh, J. Mun, and M. Jung, "A team formation model based on knowledge and collaboration," *Expert Systems with Applications*, vol. 36, no. 5, pp. 9121–9134, 2009.
- [9] C. Zhu, H. Zhu, H. Xiong, P. Ding, and F. Xie, "Recruitment market trend analysis with sequential latent variable models," in *Proceedings of the 22nd ACM SIGKDD international conference on knowledge discovery and data mining*, 2016, pp. 383–392.
- [10] Q. Zhang, H. Zhu, Y. Sun, H. Liu, F. Zhuang, and H. Xiong, "Talent demand forecasting with attentive neural sequential model," in *Proceedings of the 27th ACM SIGKDD Conference on Knowledge Discovery & Data Mining*, 2021, pp. 3906–3916.
- [11] S. E. Jackson and R. S. Schuler, "Understanding human resource management in the context of organizations and their environments," *Annual review of psychology*, vol. 46, no. 1, pp. 237–264, 1995.
- [12] N. Mathys and H. LaVan, "A survey of the human resource information systems (hris) of major companies," *Human Resource Planning*, vol. 5, no. 2, pp. 83–90, 1982.
- [13] C. Boon, D. N. Den Hartog, and D. P. Lepak, "A systematic review of human resource management systems and their measurement," *Journal of management*, vol. 45, no. 6, pp. 2498–2537, 2019.
- [14] J. B. Arthur, "Effects of human resource systems on manufacturing performance and turnover," *Academy of Management journal*, vol. 37, no. 3, pp. 670–687, 1994.
- [15] B. Gerhart, P. M. Wright, G. C. MC MAHAN, and S. A. Snell, "Measurement error in research on human resources and firm performance: how much error is there and how does it influence effect size estimates?" *Personnel psychology*, vol. 53, no. 4, pp. 803–834, 2000.
- [16] G. DeSanctis, "Human resource information systems: A current assessment," *MIS quarterly*, pp. 15–27, 1986.
- [17] R. Broderick and J. W. Boudreau, "Human resource management, information technology, and the competitive edge," *Academy of Management Perspectives*, vol. 6, no. 2, pp. 7–17, 1992.
- [18] K. S. Ball, "The use of human resource information systems: a survey," *Personnel review*, vol. 30, no. 6, pp. 677–693, 2001.
- [19] L. M. Gierminda, F. Strich, O. Christ, U. Leicht-Deobald, and A. Redzepi, "The dark sides of people analytics: reviewing the perils for organisations and employees," *European Journal of Information Systems*, vol. 31, no. 3, pp. 410–435, 2022.
- [20] U. Leicht-Deobald, T. Busch, C. Schank, A. Weibel, S. Schaffheitle, I. Wildhaber, and G. Kasper, "The challenges of algorithm-based hr decision-making for personal integrity," in *Business and the Ethical Implications of Technology*. Springer, 2022, pp. 71–86.
- [21] N. Bunker, "January 2022 jolts report: Workers quitting jobs at elevated rates," <https://www.hiringlab.org/2022/03/09/january-2022-jolts-report/>, 2022.
- [22] LinkedIn, "About linkedin," <https://about.linkedin.com>, 2022.
- [23] P. VARDALIER, "Digital transformation of human resource management: digital applications and strategic tools in hrm," pp. 239–264, 2020.
- [24] S. Bian, W. X. Zhao, Y. Song, T. Zhang, and J.-R. Wen, "Domain adaptation for person-job fit with transferable deep global match network," in *Proceedings of the 2019 Conference on Empirical Methods in Natural Language Processing and the 9th International Joint Conference on Natural Language Processing (EMNLP-IJCNLP)*, 2019, pp. 4810–4820.
- [25] Y. Sun, F. Zhuang, H. Zhu, X. Song, Q. He, and H. Xiong, "The impact of person-organization fit on talent management: A structure-aware convolutional neural network approach," in *Proceedings of the 25th ACM SIGKDD International Conference on Knowledge Discovery & Data Mining*, 2019, pp. 1625–1633.
- [26] Sun, Ying and Zhuang, Fuzhen and Zhu, Hengshu and Song, Xin and He, Qing and Xiong, Hui, "Modeling the impact of person-organization fit on talent management with structure-aware attentive neural networks," *IEEE Transactions on Knowledge & Data Engineering*, 2021.
- [27] H. Lin, H. Zhu, Y. Zuo, C. Zhu, J. Wu, and H. Xiong, "Collaborative company profiling: Insights from an employee's perspective," in *Thirty-First AAAI Conference on Artificial Intelligence*, 2017.
- [28] H. Lin, H. Zhu, J. Wu, Y. Zuo, C. Zhu, and H. Xiong, "Enhancing employer brand evaluation with collaborative topic regression models," *ACM Transactions on Information Systems (TOIS)*, vol. 38, no. 4, pp. 1–33, 2020.
- [29] M. Papachristou and Y. Yuan, "Network formation and dynamics among multi-llms," *arXiv preprint arXiv:2402.10659*, 2024.
- [30] H. Benbya, S. Pachidi, and S. Jarvenpaa, "Special issue editorial: Artificial intelligence in organizations: Implications for information systems research," *Journal of the Association for Information Systems*, vol. 22, no. 2, p. 10, 2021.
- [31] D. Shen, C. Qin, H. Zhu, T. Xu, E. Chen, and H. Xiong, "Joint representation learning with relation-enhanced topic models for intelligent job interview assessment," *ACM Transactions on Information Systems (TOIS)*, vol. 40, no. 1, pp. 1–36, 2021.
- [32] J. Chen, L. Gao, and Z. Tang, "Information extraction from resume documents in pdf format," *Electronic Imaging*, vol. 28, pp. 1–8, 2016.
- [33] K. Yao, J. Zhang, C. Qin, X. Song, P. Wang, H. Zhu, and H. Xiong, "Resuformer: Semantic structure understanding for resumes via multi-

- modal pre-training," in *2023 IEEE 39th International Conference on Data Engineering (ICDE)*. IEEE, 2023.
- [34] K. Yao, C. Qin, H. Zhu, C. Ma, J. Zhang, Y. Du, and H. Xiong, "An interactive neural network approach to keyphrase extraction in talent recruitment," in *Proceedings of the 30th ACM International Conference on Information & Knowledge Management*, 2021, pp. 2383–2393.
- [35] A. Pena, I. Serna, A. Morales, and J. Fierrez, "Bias in multimodal ai: Testbed for fair automatic recruitment," in *Proceedings of the IEEE/CVF Conference on Computer Vision and Pattern Recognition Workshops*, 2020, pp. 28–29.
- [36] C. Zhu, H. Zhu, H. Xiong, C. Ma, F. Xie, P. Ding, and P. Li, "Person-job fit: Adapting the right talent for the right job with joint representation learning," *ACM Transactions on Management Information Systems (TMIS)*, vol. 9, no. 3, pp. 1–17, 2018.
- [37] C. Zhang and H. Wang, "Resumevis: A visual analytics system to discover semantic information in semi-structured resume data," *ACM Transactions on Intelligent Systems and Technology (TIST)*, vol. 10, no. 1, pp. 1–25, 2018.
- [38] Q. Meng, H. Zhu, K. Xiao, L. Zhang, and H. Xiong, "A hierarchical career-path-aware neural network for job mobility prediction," in *Proceedings of the 25th ACM SIGKDD International Conference on Knowledge Discovery & Data Mining*, 2019, pp. 14–24.
- [39] Y. Dai, J. Qi, and R. Zhang, "Joint recognition of names and publications in academic homepages," in *Proceedings of the 13th International Conference on Web Search and Data Mining*, 2020, pp. 133–141.
- [40] V. Mittal, P. Mehta, D. Relan, and G. Gabrani, "Methodology for resume parsing and job domain prediction," *Journal of Statistics and Management Systems*, vol. 23, no. 7, pp. 1265–1274, 2020.
- [41] C. Qin, H. Zhu, T. Xu, C. Zhu, C. Ma, E. Chen, and H. Xiong, "An enhanced neural network approach to person-job fit in talent recruitment," *ACM Transactions on Information Systems (TOIS)*, vol. 38, no. 2, pp. 1–33, 2020.
- [42] C. Qin, H. Zhu, C. Zhu, T. Xu, F. Zhuang, C. Ma, J. Zhang, and H. Xiong, "Duerquiz: A personalized question recommender system for intelligent job interview," in *Proceedings of the 25th ACM SIGKDD International Conference on Knowledge Discovery & Data Mining*, 2019, pp. 2165–2173.
- [43] C. Qin, H. Zhu, D. Shen, Y. Sun, K. Yao, P. Wang, and H. Xiong, "Automatic skill-oriented question generation and recommendation for intelligent job interviews," *ACM Transactions on Information Systems*, vol. 42, no. 1, pp. 1–32, 2023.
- [44] M. Li, X. Chen, W. Liao, Y. Song, T. Zhang, D. Zhao, and R. Yan, "Ez-interviewer: To improve job interview performance with mock interview generator," in *Proceedings of the Sixteenth ACM International Conference on Web Search and Data Mining*, 2023, pp. 1102–1110.
- [45] K. Kenthapadi, A. Chudhary, and S. Ambler, "Linkedin salary: A system for secure collection and presentation of structured compensation insights to job seekers," in *2017 IEEE Symposium on Privacy-Aware Computing (PAC)*. IEEE, 2017, pp. 13–24.
- [46] Q. Meng, H. Zhu, K. Xiao, and H. Xiong, "Intelligent salary benchmarking for talent recruitment: A holistic matrix factorization approach," in *2018 IEEE International Conference on Data Mining (ICDM)*. IEEE, 2018, pp. 337–346.
- [47] T. Xu, H. Zhu, C. Zhu, P. Li, and H. Xiong, "Measuring the popularity of job skills in recruitment market: A multi-criteria approach," in *Proceedings of the AAAI Conference on Artificial Intelligence*, vol. 32, no. 1, 2018.
- [48] Y. Sun, F. Zhuang, H. Zhu, Q. Zhang, Q. He, and H. Xiong, "Market-oriented job skill valuation with cooperative composition neural network," *Nature communications*, vol. 12, no. 1, pp. 1–12, 2021.
- [49] D. Shen, H. Zhu, C. Zhu, T. Xu, C. Ma, and H. Xiong, "A joint learning approach to intelligent job interview assessment," in *IJCAI*, vol. 18, 2018, pp. 3542–3548.
- [50] L. Chen, G. Feng, C. W. Leong, B. Lehman, M. Martin-Raugh, H. Kell, C. M. Lee, and S.-Y. Yoon, "Automated scoring of interview videos using doc2vec multimodal feature extraction paradigm," in *Proceedings of the 18th ACM International Conference on Multimodal Interaction*, 2016, pp. 161–168.
- [51] L. Hemamou, G. Felhi, V. Vandenbussche, J.-C. Martin, and C. Clavel, "Hirenet: A hierarchical attention model for the automatic analysis of asynchronous video job interviews," in *Proceedings of the AAAI conference on artificial intelligence*, vol. 33, no. 01, 2019, pp. 573–581.
- [52] K. Chen, M. Niu, and Q. Chen, "A hierarchical reasoning graph neural network for the automatic scoring of answer transcripts in video job interviews," *arXiv preprint arXiv:2012.11960*, 2020.
- [53] A. Qutub, A. Al-Mehmadi, M. Al-Hssan, R. Aljohani, and H. S. Alghamdi, "Prediction of employee attrition using machine learning and ensemble methods," *Int. J. Mach. Learn. Comput.*, vol. 11, no. 2, pp. 110–114, 2021.
- [54] A. A. Mahmoud, T. A. Shawabkeh, W. A. Salameh, and I. Al Amro, "Performance predicting in hiring process and performance appraisals using machine learning," in *2019 10th International Conference on Information and Communication Systems (ICICS)*. IEEE, 2019, pp. 110–115.
- [55] Y. Ye, H. Zhu, T. Xu, F. Zhuang, R. Yu, and H. Xiong, "Identifying high potential talent: A neural network based dynamic social profiling approach," in *2019 IEEE International Conference on Data Mining (ICDM)*. IEEE, 2019, pp. 718–727.
- [56] M. Teng, H. Zhu, C. Liu, C. Zhu, and H. Xiong, "Exploiting the contagious effect for employee turnover prediction," in *Proceedings of the AAAI Conference on Artificial Intelligence*, vol. 33, no. 01, 2019, pp. 1166–1173.
- [57] J. Hang, Z. Dong, H. Zhao, X. Song, P. Wang, and H. Zhu, "Outside in: Market-aware heterogeneous graph neural network for employee turnover prediction," in *Proceedings of the Fifteenth ACM International Conference on Web Search and Data Mining*, 2022, pp. 353–362.
- [58] C. Wang, H. Zhu, C. Zhu, X. Zhang, E. Chen, and H. Xiong, "Personalized employee training course recommendation with career development awareness," in *Proceedings of the Web Conference 2020*, 2020, pp. 1648–1659.
- [59] R. Srivastava, G. K. Palshikar, S. Chaurasia, and A. Dixit, "What's next? a recommendation system for industrial training," *Data Science and Engineering*, vol. 3, no. 3, pp. 232–247, 2018.
- [60] J. Li, Y. Long, T. Wang, D. Shen, and Z. Zhang, "A data-driven method for competency evaluation of personnel," in *Proceedings of the 3rd International Conference on Data Science and Information Technology*, 2020, pp. 93–104.
- [61] H. Liu, S. Dai, and H. Jiang, "Application of rough set and support vector machine in competency assessment," in *2009 Fourth International Conference on Bio-Inspired Computing*. IEEE, 2009, pp. 1–4.
- [62] D. S. Pugh, "Organization theory: selected classic readings," 2007.
- [63] J. Klünder, J. Horstmann, and O. Karras, "Identifying the mood of a software development team by analyzing text-based communication in chats with machine learning," in *International Conference on Human-Centred Software Engineering*. Springer, 2020, pp. 133–151.
- [64] H. Cao, V. Yang, V. Chen, Y. J. Lee, L. Stone, N. J. Diarrassouba, M. E. Whiting, and M. S. Bernstein, "My team will go on: Differentiating high and low viability teams through team interaction," *Proceedings of the ACM on Human-Computer Interaction*, vol. 4, no. CSCW3, pp. 1–27, 2021.
- [65] M. Teng, H. Zhu, C. Liu, and H. Xiong, "Exploiting network fusion for organizational turnover prediction," *ACM Transactions on Management Information Systems (TMIS)*, vol. 12, no. 2, pp. 1–18, 2021.
- [66] V. Ikoro, M. Sharmina, K. Malik, and R. Batista-Navarro, "Analyzing sentiments expressed on twitter by uk energy company consumers," in *2018 Fifth international conference on social networks analysis, management and security (SNAMS)*. IEEE, 2018, pp. 95–98.
- [67] R. Spears, "The impact of public opinion on large global companies' market valuations: A markov switching model approach," *Journal of Finance and Economics*, vol. 9, no. 3, pp. 115–141, 2021.
- [68] R. Bajpai, D. Hazarika, K. Singh, S. Gorantla, E. Cambria, and R. Zimmerman, "Aspect-sentiment embeddings for company profiling and employee opinion mining," *arXiv preprint arXiv:1902.08342*, 2019.
- [69] T. Schmiedel, O. Müller, and J. vom Brocke, "Topic modeling as a strategy of inquiry in organizational research: A tutorial with an application example on organizational culture," *Organizational Research Methods*, vol. 22, no. 4, pp. 941–968, 2019.
- [70] J. Park, I. B. Wood, E. Jing, A. Nematzadeh, S. Ghosh, M. D. Conover, and Y.-Y. Ahn, "Global labor flow network reveals the hierarchical organization and dynamics of geo-industrial clusters," *Nature communications*, vol. 10, no. 1, pp. 1–10, 2019.
- [71] X. Chen, C. Qin, F. Chuyu, C. Wang, C. Zhu, F. Zhuang, H. Zhu, and H. Xiong, "Job-sdf: A multi-granularity dataset for job skill demand forecasting and benchmarking," *arXiv preprint arXiv:2406.11920*, 2024.
- [72] W. F. Cascio and H. Aguinis, "Research in industrial and organizational psychology from 1963 to 2007: Changes, choices, and trends," *Journal of Applied Psychology*, vol. 93, no. 5, p. 1062, 2008.
- [73] C. Qin, K. Yao, H. Zhu, T. Xu, D. Shen, E. Chen, and H. Xiong, "Towards automatic job description generation with capability-aware neural networks," *IEEE Transactions on Knowledge and Data Engineering*, 2022.
- [74] V. Ha-Thuc, Y. Yan, X. Wu, V. Dialani, A. Gupta, and S. Sinha, "From query-by-keyword to query-by-example: LinkedIn talent search approach," in *Proceedings of the 2017 ACM on Conference on Information and Knowledge Management*, 2017, pp. 1737–1745.
- [75] O. Manad, M. Bentounsi, and P. Darmon, "Enhancing talent search by integrating and querying big hr data," in *2018 IEEE International Conference on Big Data (Big Data)*. IEEE, 2018, pp. 4095–4100.
- [76] P. Gupta, S. F. Fernandes, and M. Jain, "Automation in recruitment: a new frontier," *Journal of Information Technology Teaching Cases*, vol. 8, no. 2, pp. 118–125, 2018.
- [77] B. Shi, S. Li, J. Yang, M. E. Kazdagli, and Q. He, "Learning to ask screening questions for job postings," in *Proceedings of the 43rd International ACM SIGIR Conference on Research and Development in Information Retrieval*, 2020, pp. 549–558.
- [78] Y. Zhao, M. K. Hryniewicki, F. Cheng, B. Fu, and X. Zhu, "Employee turnover prediction with machine learning: A reliable approach," in *Proceedings of SAI intelligent systems conference*. Springer, 2018, pp. 737–758.
- [79] Y. Long, J. Liu, M. Fang, T. Wang, and W. Jiang, "Prediction of employee promotion based on personal basic features and post features," in *Proceedings of the International Conference on Data Processing and Applications*, 2018, pp. 5–10.
- [80] L. Liu, J. Liu, W. Zhang, Z. Chi, W. Shi, and Y. Huang, "Hiring now: A skill-aware multi-attention model for job posting generation," in *Proceedings of the 58th Annual Meeting of the Association for Computational Linguistics*, 2020, pp. 3096–3104.
- [81] A. Lorincz, D. Graus, D. Lavi, and J. L. M. Pereira, "Transfer learning for multilingual vacancy text generation," in *Proceedings of the 2nd Workshop on Natural Language Generation, Evaluation, and Metrics (GEM)*, 2022, pp. 207–222.
- [82] C. Borchers, D. Gala, B. Gilbert, E. Oravkin, W. Bounsi, Y. M. Asano, and H. Kirk, "Looking for a handsome carpenter! debiasing gpt-3 job advertisements," in *Proceedings of the 4th Workshop on Gender Bias in Natural Language Processing (GeBNLP)*, 2022, pp. 212–224.
- [83] S. Böhm, O. Linnyk, J. Kohl, T. Weber, I. Teetz, K. Bandurka, and M. Kersting, "Analysing gender bias in it job postings: A pre-study based on samples from the german job market," in *Proceedings of the 2020 on computers*

- and people research conference, 2020, pp. 72–80.
- [84] R. Mao, L. Tan, and R. Moieni, “Developing a large-scale language model to unveil and alleviate gender and age biases in australian job ads,” in *2023 IEEE International Conference on Big Data (BigData)*. IEEE, 2023, pp. 4176–4185.
  - [85] F. Gilardi, M. Alizadeh, and M. Kubli, “Chatgpt outperforms crowd workers for text-annotation tasks,” *Proceedings of the National Academy of Sciences*, vol. 120, no. 30, p. e2305016120, 2023.
  - [86] X. Chen, C. Qin, Z. Wang, Y. Cheng, C. Wang, H. Zhu, and H. Xiong, “Pre-dygae: Pre-training enhanced dynamic graph autoencoder for occupational skill demand forecasting,” in *IJCAI*, 2024.
  - [87] J. Chen, D. Zhu, X. Shen, X. Li, Z. Liu, P. Zhang, R. Krishnamoorthi, V. Chandra, Y. Xiong, and M. Elhoseiny, “Minigpt-v2: large language model as a unified interface for vision-language multi-task learning,” *arXiv preprint arXiv:2310.09478*, 2023.
  - [88] V. Ha-Thuc, Y. Xu, S. P. Kanduri, X. Wu, V. Dialani, Y. Yan, A. Gupta, and S. Sinha, “Search by ideal candidates: Next generation of talent search at linkedin,” in *Proceedings of the 25th International Conference Companion on World Wide Web*, 2016, pp. 195–198.
  - [89] S. K. Koppurapu, “Automatic extraction of usable information from unstructured resumes to aid search,” in *2010 IEEE International Conference on Progress in Informatics and Computing*, vol. 1. IEEE, 2010, pp. 99–103.
  - [90] K. Yu, G. Guan, and M. Zhou, “Resume information extraction with cascaded hybrid model,” in *Proceedings of the 43rd annual meeting of the Association for Computational Linguistics (ACL’05)*, 2005, pp. 499–506.
  - [91] C. Ayishathahira, C. Sreejith, and C. Raseek, “Combination of neural networks and conditional random fields for efficient resume parsing,” in *2018 International CET Conference on Control, Communication, and Computing (IC4)*. IEEE, 2018, pp. 388–393.
  - [92] L. Pham Van, S. Vu Ngoc, and V. Nguyen Van, “Study of information extraction in resume,” Conference, 2018.
  - [93] Y. Jin, J. Xie, W. Guo, C. Luo, D. Wu, and R. Wang, “Lstm-crf neural network with gated self attention for chinese ner,” *IEEE Access*, vol. 7, pp. 136 694–136 703, 2019.
  - [94] X. Li, H. Shu, Y. Zhai, and Z. Lin, “A method for resume information extraction using bert-bilstm-crf,” in *2021 IEEE 21st International Conference on Communication Technology (ICCT)*. IEEE, 2021, pp. 1437–1442.
  - [95] M. Wei, Y. He, and Q. Zhang, “Robust layout-aware ie for visually rich documents with pre-trained language models,” in *Proceedings of the 43rd International ACM SIGIR Conference on Research and Development in Information Retrieval*, 2020, pp. 2367–2376.
  - [96] F. Jiang, C. Qin, J. Zhang, K. Yao, X. Chen, D. Shen, C. Zhu, H. Zhu, and H. Xiong, “Towards efficient resume understanding: A multi-granularity multi-modal pre-training approach,” 2024.
  - [97] Y. Xu, T. Lv, L. Cui, G. Wang, Y. Lu, D. Florencio, C. Zhang, and F. Wei, “Layoutlm: Multimodal pre-training for multilingual visually-rich document understanding,” *arXiv preprint arXiv:2104.08836*, 2021.
  - [98] Y. Xu, M. Li, L. Cui, S. Huang, F. Wei, and M. Zhou, “Layoutlm: Pre-training of text and layout for document image understanding,” in *Proceedings of the 26th ACM SIGKDD international conference on knowledge discovery & data mining*, 2020, pp. 1192–1200.
  - [99] Y. Wang, Y. Allouache, and C. Joubert, “Analysing cv corpus for finding suitable candidates using knowledge graph and bert,” in *DBKDA 2021, The Thirteenth International Conference on Advances in Databases, Knowledge, and Data Applications*, 2021.
  - [100] A. Apatean, E. Szakacs, and M. Tilca, “Machine-learning based application for staff recruiting,” *Acta Technica Napocensis*, vol. 58, no. 4, pp. 16–21, 2017.
  - [101] C. Ozcaglar, S. Geyik, B. Schmitz, P. Sharma, A. Shelkovnykov, Y. Ma, and E. Buchanan, “Entity personalized talent search models with tree interaction features,” in *The World Wide Web Conference*, 2019, pp. 3116–3122.
  - [102] S. C. Geyik, V. Dialani, M. Meng, and R. Smith, “In-session personalization for talent search,” in *Proceedings of the 27th ACM International Conference on Information and Knowledge Management*, 2018, pp. 2107–2115.
  - [103] R. Ramanath, H. Inan, G. Polatkan, B. Hu, Q. Guo, C. Ozcaglar, X. Wu, K. Kenthapadi, and S. C. Geyik, “Towards deep and representation learning for talent search at linkedin,” in *Proceedings of the 27th ACM international conference on information and knowledge management*, 2018, pp. 2253–2261.
  - [104] Z. Yang, S. Yan, A. Lad, X. Liu, and W. Guo, “Cascaded deep neural ranking models in linkedin people search,” in *Proceedings of the 30th ACM International Conference on Information & Knowledge Management*, 2021, pp. 4312–4320.
  - [105] Y. Zhang, B. Liu, and J. Qian, “Fedpjl: federated contrastive learning for privacy-preserving person-job fit,” *Applied Intelligence*, vol. 53, no. 22, pp. 27 060–27 071, 2023.
  - [106] Y. Saito and K. Sugiyama, “Multi-behavior job recommendation with dynamic availability,” in *Proceedings of the Annual International ACM SIGIR Conference on Research and Development in Information Retrieval in the Asia Pacific Region*, 2023, pp. 264–271.
  - [107] B. Fu, H. Liu, Y. Zhu, Y. Song, T. Zhang, and Z. Wu, “Beyond matching: Modeling two-sided multi-behavioral sequences for dynamic person-job fit,” in *International Conference on Database Systems for Advanced Applications*. Springer, 2021, pp. 359–375.
  - [108] J. Malinowski, T. Keim, O. Wendt, and T. Weitzel, “Matching people and jobs: A bilateral recommendation approach,” in *Proceedings of the 39th Annual Hawaii International Conference on System Sciences (HICSS’06)*, vol. 6. IEEE, 2006, pp. 137c–137c.
  - [109] J. Zhao, J. Wang, M. Sigdel, B. Zhang, P. Hoang, M. Liu, and M. Korayem, “Embedding-based recommender system for job to candidate matching on scale,” *arXiv preprint arXiv:2107.00221*, 2021.
  - [110] Z. Wang, W. Wei, C. Xu, J. Xu, and X.-L. Mao, “Person-job fit estimation from candidate profile and related recruitment history with co-attention neural networks,” *Neurocomputing*, vol. 501, pp. 14–24, 2022.
  - [111] Y. Luo, H. Zhang, Y. Wen, and X. Zhang, “Resumegan: An optimized deep representation learning framework for talent-job fit via adversarial learning,” in *Proceedings of the 28th ACM International Conference on Information and Knowledge Management*, 2019, pp. 1101–1110.
  - [112] D. Lavi, V. Medentsiy, and D. Graus, “consultantbert: Fine-tuned siamese sentence-bert for matching jobs and job seekers,” *arXiv preprint arXiv:2109.06501*, 2021.
  - [113] E. Abdollahnejad, M. Kalman, and B. H. Far, “A deep learning bert-based approach to person-job fit in talent recruitment,” in *2021 International Conference on Computational Science and Computational Intelligence (CSCI)*. IEEE, 2021, pp. 98–104.
  - [114] H. Liu and Y. Ge, “Job and employee embeddings: A joint deep learning approach,” *IEEE Transactions on Knowledge and Data Engineering*, 2022.
  - [115] M. Kaya and T. Bogers, “An exploration of sentence-pair classification for algorithmic recruiting,” in *Proceedings of the 17th ACM Conference on Recommender Systems*, 2023, pp. 1175–1179.
  - [116] C. Fang, C. Qin, Q. Zhang, K. Yao, J. Zhang, H. Zhu, F. Zhuang, and H. Xiong, “Recruitpro: A pretrained language model with skill-aware prompt learning for intelligent recruitment,” in *Proceedings of the 29th ACM SIGKDD International Conference on Knowledge Discovery and Data Mining (SIGKDD-2023)*, 2023.
  - [117] S. Bian, X. Chen, W. X. Zhao, K. Zhou, Y. Hou, Y. Song, T. Zhang, and J.-R. Wen, “Learning to match jobs with resumes from sparse interaction data using multi-view co-teaching network,” in *Proceedings of the 29th ACM International Conference on Information & Knowledge Management*, 2020, pp. 65–74.
  - [118] X. Yu, J. Zhang, and Z. Yu, “Confit: Improving resume-job matching using data augmentation and contrastive learning,” *arXiv preprint arXiv:2401.16349*, 2024.
  - [119] J. Jiang, S. Ye, W. Wang, J. Xu, and X. Luo, “Learning effective representations for person-job fit by feature fusion,” in *Proceedings of the 29th ACM International Conference on Information & Knowledge Management*, 2020, pp. 2549–2556.
  - [120] M. He, T. Wang, Y. Zhu, Y. Chen, F. Yao, and N. Wang, “Finn: Feature interaction neural network for person-job fit,” in *2021 7th International Conference on Big Data and Information Analytics (BigDIA)*. IEEE, 2021, pp. 123–130.
  - [121] M. He, D. Shen, T. Wang, H. Zhao, Z. Zhang, and R. He, “Self-attentional multi-field features representation and interaction learning for person-job fit,” *IEEE Transactions on Computational Social Systems*, 2021.
  - [122] Y. Hou, X. Pan, W. X. Zhao, S. Bian, Y. Song, T. Zhang, and J.-R. Wen, “Leveraging search history for improving person-job fit,” in *International Conference on Database Systems for Advanced Applications*. Springer, 2022, pp. 38–54.
  - [123] B. Fu, H. Liu, H. Zhao, Y. Zhu, Y. Song, T. Zhang, and Z. Wu, “Market-aware dynamic person-job fit with hierarchical reinforcement learning,” in *International Conference on Database Systems for Advanced Applications*. Springer, 2022, pp. 697–705.
  - [124] D. Shen, H. Zhu, K. Xiao, X. Zhang, and H. Xiong, “Exploiting connections among personality, job position, and work behavior: Evidence from joint bayesian learning,” *ACM Transactions on Management Information Systems*, vol. 14, no. 3, pp. 1–20, 2023.
  - [125] E. Faliagka, L. Iliadis, I. Karydis, M. Rigou, S. Sioutas, A. Tsakalidis, and G. Tzimas, “On-line consistent ranking on e-recruitment: seeking the truth behind a well-formed cv,” *Artificial Intelligence Review*, vol. 42, no. 3, pp. 515–528, 2014.
  - [126] P. Van Esch, J. S. Black, and J. Ferolie, “Marketing ai recruitment: The next phase in job application and selection,” *Computers in Human Behavior*, vol. 90, pp. 215–222, 2019.
  - [127] X. Yu, C. Qin, Q. Zhang, C. Zhu, H. Ma, X. Zhang, and H. Zhu, “Disco: A hierarchical disentangled cognitive diagnosis framework for interpretable job recommendation,” in *2024 IEEE International Conference on Data Mining (ICDM)*. IEEE, 2024.
  - [128] C. Yang, Y. Hou, Y. Song, T. Zhang, J.-R. Wen, and W. X. Zhao, “Modeling two-way selection preference for person-job fit,” in *Proceedings of the 16th ACM Conference on Recommender Systems*, 2022, pp. 102–112.
  - [129] H. Zhao, X. Wu, C. Zhao, L. Zhang, H. Ma, and F. Cheng, “Coea: A cooperative-competitive evolutionary algorithm for bidirectional recommendations,” *IEEE Transactions on Evolutionary Computation*, vol. 26, no. 1, pp. 28–42, 2021.
  - [130] D. Ntioudis, P. Masa, A. Karakostas, G. Meditskos, S. Vrochidis, and I. Kompatsiaris, “Ontology-based personalized job recommendation framework for migrants and refugees,” *Big Data and Cognitive Computing*, vol. 6, no. 4, p. 120, 2022.
  - [131] Y. Zhang, B. Liu, J. Qian, J. Qin, X. Zhang, and X. Jiang, “An explainable person-job fit model incorporating structured information,” in *2021 IEEE International Conference on Big Data (Big Data)*. IEEE, 2021, pp. 3571–3579.
  - [132] A. Cardoso, F. Mourão, and L. Rocha, “The matching scarcity problem: When recommenders do not connect the edges in recruitment services,” *Expert Systems with Applications*, vol. 175, p. 114764, 2021.
  - [133] Y. Mashayekhi, B. Kang, J. Lijffijt, and T. De Bie, “Recon: Reducing conges-

- tion in job recommendation using optimal transport," in *Proceedings of the 17th ACM Conference on Recommender Systems*, 2023, pp. 696–701.
- [134] D. Kumar, T. Grosz, N. Rekabsaz, E. Greif, and M. Schedl, "Fairness of recommender systems in the recruitment domain: an analysis from technical and legal perspectives," *Frontiers in big Data*, vol. 6, 2023.
- [135] Z. Zheng, Z. Qiu, X. Hu, L. Wu, H. Zhu, and H. Xiong, "Generative job recommendations with large language model," *arXiv preprint arXiv:2307.02157*, 2023.
- [136] Y. Du, D. Luo, R. Yan, X. Wang, H. Liu, H. Zhu, Y. Song, and J. Zhang, "Enhancing job recommendation through llm-based generative adversarial networks," in *Proceedings of the AAAI Conference on Artificial Intelligence*, vol. 38, no. 8, 2024, pp. 8363–8371.
- [137] S. Datta, P. Mallick, S. Patil, I. Bhattacharya, and G. Palshikar, "Generating an optimal interview question plan using a knowledge graph and integer linear programming," in *Proceedings of the 2021 Conference of the North American Chapter of the Association for Computational Linguistics: Human Language Technologies*, 2021, pp. 1996–2005.
- [138] S. Pal, K. Khan, A. K. Singh, S. Ghosh, T. Nayak, G. Palshikar, and I. Bhattacharya, "Weakly supervised context-based interview question generation," in *Proceedings of the 2nd Workshop on Natural Language Generation, Evaluation, and Metrics (GEM)*, 2022, pp. 43–53.
- [139] F. Jiang, C. Qin, K. Yao, C. Fang, F. Zhuang, H. Zhu, and H. Xiong, "Enhancing question answering for enterprise knowledge bases using large language models," in *Proceedings of the 29th International Conference on Database Systems for Advanced Applications (DASFAA 2024)*, 2024.
- [140] H. Ma, Y. Zeng, S. Yang, C. Qin, X. Zhang, and L. Zhang, "A novel computerized adaptive testing framework with decoupled learning selector," *Complex & Intelligent Systems*, vol. 9, no. 5, pp. 5555–5566, 2023.
- [141] I. Naim, M. I. Tanveer, D. Gildea, and M. E. Hoque, "Automated prediction and analysis of job interview performance: The role of what you say and how you say it," in *2015 11th IEEE international conference and workshops on automatic face and gesture recognition (FG)*, vol. 1. IEEE, 2015, pp. 1–6.
- [142] L. Chen, R. Zhao, C. W. Leong, B. Lehman, G. Feng, and M. E. Hoque, "Automated video interview judgment on a large-sized corpus collected online," in *2017 Seventh International Conference on Affective Computing and Intelligent Interaction (ACII)*. IEEE, 2017, pp. 504–509.
- [143] L. Hemamou, G. Felhi, J.-C. Martin, and C. Clavel, "Slices of attention in asynchronous video job interviews," in *2019 8th International Conference on Affective Computing and Intelligent Interaction (ACII)*. IEEE, 2019, pp. 1–7.
- [144] L. S. Nguyen, D. Frauendorfer, M. S. Mast, and D. Gatica-Perez, "Hire me: Computational inference of hirability in employment interviews based on nonverbal behavior," *IEEE transactions on multimedia*, vol. 16, no. 4, pp. 1018–1031, 2014.
- [145] A. Singhanian, A. Unnam, and V. Aggarwal, "Grading video interviews with fairness considerations," *arXiv preprint arXiv:2007.05461*, 2020.
- [146] L. Hemamou, A. Guillon, J.-C. Martin, and C. Clavel, "Don't judge me by my face: An indirect adversarial approach to remove sensitive information from multimodal neural representation in asynchronous job video interviews," in *2021 9th International Conference on Affective Computing and Intelligent Interaction (ACII)*. IEEE, 2021, pp. 1–8.
- [147] T. Zhang, A. Koutsoumpis, J. K. Oostrom, D. Holtrop, S. Ghassemi, and R. E. de Vries, "Can large language models assess personality from asynchronous video interviews? a comprehensive evaluation of validity, reliability, fairness, and rating patterns," *IEEE Transactions on Affective Computing*, 2024.
- [148] Y. Zhang, C. Qin, D. Shen, H. Ma, L. Zhang, X. Zhang, and H. Zhu, "Relicd: A reliable cognitive diagnosis framework with confidence awareness," in *2023 IEEE International Conference on Data Mining (ICDM)*. IEEE, 2023, pp. 858–867.
- [149] X. Yu, C. Qin, D. Shen, H. Ma, L. Zhang, X. Zhang, H. Zhu, and H. Xiong, "Rdgt: Enhancing group cognitive diagnosis with relation-guided dual-side graph transformer," *IEEE Transactions on Knowledge and Data Engineering*, 2024.
- [150] Y. Lin, F. Lin, W. Zeng, J. Xiahou, L. Li, P. Wu, Y. Liu, and C. Miao, "Hierarchical reinforcement learning with dynamic recurrent mechanism for course recommendation," *Knowledge-Based Systems*, vol. 244, p. 108546, 2022.
- [151] S. Patki, V. Sankhe, M. Jawwad, and N. Mulla, "Personalised employee training," in *2021 International Conference on Communication information and Computing Technology (ICCICT)*. IEEE, 2021, pp. 1–6.
- [152] Z. Zheng, Y. Sun, X. Song, H. Zhu, and H. Xiong, "Generative learning plan recommendation for employees: A work performance-aware reinforcement learning approach," in *Proceedings of the 17th ACM Conference on Recommender Systems*, 2023.
- [153] Y. Yang, C. Zhang, X. Song, Z. Dong, H. Zhu, and W. Li, "Contextualized knowledge graph embedding for explainable talent training course recommendation," *ACM Transactions on Information Systems*, 2023.
- [154] X. Yu, C. Qin, D. Shen, S. Yang, H. Ma, H. Zhu, and X. Zhang, "Rigl: A unified reciprocal approach for tracing the independent and group learning processes," in *Proceedings of the 30th ACM SIGKDD Conference on Knowledge Discovery and Data Mining*, 2024, pp. 4047–4058.
- [155] M. Ilwani, G. Nassreddine, and J. Younis, "Machine learning application on employee promotion," *Mesopotamian Journal of Computer Science*, vol. 2023, pp. 106–120, 2023.
- [156] K. Sahinbas, "Employee promotion prediction by using machine learning algorithms for imbalanced dataset," in *2022 2nd International Conference on Computing and Machine Intelligence (ICMI)*. IEEE, 2022, pp. 1–5.
- [157] S. Shafie, P. O. Soek, and W. K. Khai, "Prediction of employee promotion using hybrid sampling method with machine learning architecture," *Malaysian Journal of Computing (MJoC)*, vol. 8, no. 1, pp. 1264–1286, 2023.
- [158] J. Yuan, Q.-M. Zhang, J. Gao, L. Zhang, X.-S. Wan, X.-J. Yu, and T. Zhou, "Promotion and resignation in employee networks," *Physica A: Statistical Mechanics and its Applications*, vol. 444, pp. 442–447, 2016.
- [159] J. Liu, J. Huang, T. Wang, L. Xing, and R. He, "A data-driven analysis of employee development based on working expertise," *IEEE Transactions on Computational Social Systems*, vol. 8, no. 2, pp. 410–422, 2021.
- [160] A. Guarino, D. Malandrino, F. Marzullo, A. Torre, and R. Zaccagnino, "Adaptive talent journey: Optimization of talents' growth path within a company via deep q-learning," *Expert Systems with Applications*, vol. 209, p. 118302, 2022.
- [161] L. Ma, "Employee turnover prediction based on machine learning model," in *2022 5th Asia Conference on Machine Learning and Computing (ACMLC)*. IEEE, 2022, pp. 22–27.
- [162] K. Konar, S. Das, and S. Das, "Employee attrition prediction for imbalanced data using genetic algorithm-based parameter optimization of xgb classifier," in *2023 International Conference on Computer, Electrical & Communication Engineering (ICCECE)*. IEEE, 2023, pp. 1–6.
- [163] M. Gollapalli, A.-U. Rahman, A. Osama, A. Alfaify, M. Yassin, and A. Alabdullah, "Data mining and visualization to understand employee attrition and work performance," in *2023 3rd International Conference on Computing and Information Technology (ICCIT)*. IEEE, 2023, pp. 149–154.
- [164] D. Alao and A. Adeyemo, "Analyzing employee attrition using decision tree algorithms," *Computing, Information Systems, Development Informatics and Allied Research Journal*, vol. 4, no. 1, pp. 17–28, 2013.
- [165] V. Nagadevara, V. Srinivasan, and R. Valk, "Establishing a link between employee turnover and withdrawal behaviours: Application of data mining techniques," 2008.
- [166] T. Juvitayapun, "Employee turnover prediction: The impact of employee event features on interpretable machine learning methods," in *2021 13th international conference on knowledge and smart technology (kst)*. IEEE, 2021, pp. 181–185.
- [167] M. Chaudhary, L. Gaur, and A. Chakrabarti, "Comparative analysis of entropy weight method and c5 classifier for predicting employee churn," in *2022 3rd International Conference on Intelligent Engineering and Management (ICIEM)*. IEEE, 2022, pp. 232–236.
- [168] A. B. Wild Ali, "Prediction of employee turn over using random forest classifier with intensive optimized pca algorithm," *Wireless Personal Communications*, vol. 119, no. 4, pp. 3365–3382, 2021.
- [169] L. Zhang, D. Zhou, H. Zhu, T. Xu, R. Zha, E. Chen, and H. Xiong, "Attentive heterogeneous graph embedding for job mobility prediction," in *Proceedings of the 27th ACM SIGKDD Conference on Knowledge Discovery & Data Mining*, 2021, pp. 2192–2201.
- [170] B. Subha, I. A. K. Shaikh, P. J. Patil, R. Sethumadhavan, M. Preetha, and H. Patil, "Predictive analysis of employee turnover in it using a hybrid crf-bilstm and cnn model," in *2023 International Conference on Sustainable Communication Networks and Application (ICSCNA)*. IEEE, 2023, pp. 914–919.
- [171] N. Arambepola and L. Munasinghe, "What makes job satisfaction in the information technology industry?" in *2021 International Research Conference on Smart Computing and Systems Engineering (SCSE)*, vol. 4. IEEE, 2021, pp. 99–105.
- [172] K. Saha, A. Yousuf, L. Hickman, P. Gupta, L. Tay, and M. De Choudhury, "A social media study on demographic differences in perceived job satisfaction," *Proceedings of the ACM on Human-Computer Interaction*, vol. 5, no. CSCW1, pp. 1–29, 2021.
- [173] L. Saleh and S. Abu-Soud, "Predicting jordanian job satisfaction using artificial neural network and decision tree," in *2021 11th International Conference on Advanced Computer Information Technologies (ACIT)*. IEEE, 2021, pp. 735–738.
- [174] N. McJames, A. Parnell, and A. O'Shea, "Factors affecting teacher job satisfaction and retention: A causal inference machine learning approach using data from talis 2018," 2022.
- [175] G. D. Devi and S. Kamalakannan, "Prediction of job satisfaction from the employee using ensemble method," in *2022 International Conference on Advanced Computing Technologies and Applications (ICACTA)*. IEEE, 2022, pp. 1–8.
- [176] C. P. Maertz Jr and K. R. Kmita, "Integrating turnover reasons and shocks with turnover decision processes," *Journal of Vocational Behavior*, vol. 81, no. 1, pp. 26–38, 2012.
- [177] L. Li, H. Jing, H. Tong, J. Yang, Q. He, and B.-C. Chen, "Nemo: Next career move prediction with contextual embedding," in *Proceedings of the 26th International Conference on World Wide Web Companion*, 2017, pp. 505–513.
- [178] M. Yamashita, Y. Li, T. Tran, Y. Zhang, and D. Lee, "Looking further into the future: Career pathway prediction," *WSDM Computational Jobs Marketplace*, 2022.
- [179] C. Wang, H. Zhu, Q. Hao, K. Xiao, and H. Xiong, "Variable interval time sequence modeling for career trajectory prediction: Deep collaborative perspective," in *Proceedings of the Web Conference 2021*, 2021, pp. 612–623.
- [180] M. He, X. Zhan, D. Shen, Y. Zhu, H. Zhao, and R. He, "What about your next job? predicting professional career trajectory using neural networks," in *Proceedings of the 2021 4th International Conference on Machine Learning and Machine Intelligence*, 2021, pp. 184–189.
- [181] J.-J. Decorte, J. Van Haute, J. Deleu, C. Develder, and T. Demeester, "Career path prediction using resume representation learning and skill-

- based matching," *arXiv preprint arXiv:2310.15636*, 2023.
- [182] R. Zha, Y. Sun, C. Qin, L. Zhang, T. Xu, H. Zhu, and E. Chen, "Towards unified representation learning for career mobility analysis with trajectory hypergraph," *ACM Transactions on Information Systems*, 2024.
- [183] P. Guo, K. Xiao, Z. Ye, H. Zhu, and W. Zhu, "Intelligent career planning via stochastic subsampling reinforcement learning," *Scientific Reports*, vol. 12, no. 1, pp. 1–16, 2022.
- [184] Y. Sun, H. Zhu, L. Wang, L. Zhang, and H. Xiong, "Large-scale online job search behaviors reveal labor market shifts amid covid-19," *Nature Cities*, vol. 1, no. 2, pp. 150–163, 2024.
- [185] R. Schellingerhout, V. Medentsiy, and M. Marx, "Explainable career path predictions using neural models," *Recommender Systems for Human Resources*, vol. 3218, p. 7, 2022.
- [186] R. Duncan, "What is the right organization structure? decision tree analysis provides the answer," *Organizational dynamics*, vol. 7, no. 3, pp. 59–80, 1979.
- [187] D. Zhang, J. Liu, H. Zhu, Y. Liu, L. Wang, P. Wang, and H. Xiong, "Job2vec: Job title benchmarking with collective multi-view representation learning," in *Proceedings of the 28th ACM International Conference on Information and Knowledge Management*, 2019, pp. 2763–2771.
- [188] B. Perozzi, R. Al-Rfou, and S. Skiena, "Deepwalk: Online learning of social representations," in *Proceedings of the 20th ACM SIGKDD international conference on Knowledge discovery and data mining*, 2014, pp. 701–710.
- [189] R. Silzer and A. H. Church, "Identifying and assessing high-potential talent," *Strategy-driven talent management: A leadership imperative*, vol. 28, pp. 213–280, 2010.
- [190] J. Zenger and J. Folkman, "Companies are bad at identifying high-potential employees," *Harvard Business Review*, pp. 2–5, 2017.
- [191] J. Gelens, J. Hofmans, N. Dries, and R. Pepermans, "Talent management and organisational justice: Employee reactions to high potential identification," *Human Resource Management Journal*, vol. 24, no. 2, pp. 159–175, 2014.
- [192] D. Yin, X. Zhang, and H. Zhao, "Understanding and predicting innovative potential of scholars based on deep learning method," in *PACIS 2022 Proceedings*, 2022.
- [193] Y. Cheng, X. Tang, X. Zhang, and H. Xiong, "Effectiveness of ai in strategic decision making: An empirical study on identifying high-potential talents," in *Forty-Second International Conference on Information Systems 2021 Proceedings*, 2021.
- [194] Pugh, Derek Salman, "Organization theory: Selected readings," *Penguin (Non-Classics)*, 1971.
- [195] T. Lappas, K. Liu, and E. Terzi, "Finding a team of experts in social networks," in *Proceedings of the 15th ACM SIGKDD international conference on Knowledge discovery and data mining*, 2009, pp. 467–476.
- [196] M. Kargar, A. An, and M. Zihayat, "Efficient bi-objective team formation in social networks," in *Joint European Conference on Machine Learning and Knowledge Discovery in Databases*. Springer, 2012, pp. 483–498.
- [197] M. Zihayat, A. An, L. Golab, M. Kargar, and J. Szlichta, "Authority-based team discovery in social networks," *arXiv preprint arXiv:1611.02992*, 2016.
- [198] X. Wang, Z. Zhao, and W. Ng, "Ustf: a unified system of team formation," *IEEE Transactions on Big Data*, vol. 2, no. 1, pp. 70–84, 2016.
- [199] R. Hamidi Rad, H. Fani, M. Kargar, J. Szlichta, and E. Bagheri, "Learning to form skill-based teams of experts," in *Proceedings of the 29th ACM International Conference on Information & Knowledge Management*, 2020, pp. 2049–2052.
- [200] R. Hamidi Rad, H. Fani, E. Bagheri, M. Kargar, D. Srivastava, and J. Szlichta, "A variational neural architecture for skill-based team formation," *ACM Transactions on Information Systems*, vol. 42, no. 1, pp. 1–28, 2023.
- [201] H. Fani, R. Barzegar, A. Dashti, and M. Saeedi, "A streaming approach to neural team formation training," in *European Conference on Information Retrieval*. Springer, 2024, pp. 325–340.
- [202] A. Dashti, S. Samet, and H. Fani, "Effective neural team formation via negative samples," in *Proceedings of the 31st ACM International Conference on Information & Knowledge Management*, 2022, pp. 3908–3912.
- [203] Q. Liu, T. Luo, R. Tang, and S. Bressan, "An efficient and truthful pricing mechanism for team formation in crowdsourcing markets," in *2015 IEEE International Conference on Communications (ICC)*. IEEE, 2015, pp. 567–572.
- [204] G. Barnabò, A. Fazzzone, S. Leonardi, and C. Schwiegelshohn, "Algorithms for fair team formation in online labour marketplaces," in *Companion Proceedings of The 2019 World Wide Web Conference*, 2019, pp. 484–490.
- [205] A. Anagnostopoulos, C. Castillo, A. Fazzzone, S. Leonardi, and E. Terzi, "Algorithms for hiring and outsourcing in the online labor market," in *Proceedings of the 24th ACM SIGKDD International Conference on Knowledge Discovery & Data Mining*, 2018, pp. 1109–1118.
- [206] J. Nemec, H. Davoudi, L. Golab, M. Kargar, Y. Lytyyn, P. Mierzejewski, J. Szlichta, and M. Zihayat, "Rw-team: Robust team formation using random walk," in *Proceedings of the 30th ACM International Conference on Information & Knowledge Management*, 2021, pp. 4759–4763.
- [207] L. Li, H. Tong, N. Cao, K. Ehrlich, Y.-R. Lin, and N. Buchler, "Replacing the irreplaceable: Fast algorithms for team member recommendation," in *Proceedings of the 24th International Conference on World Wide Web*, 2015, pp. 636–646.
- [208] Li, Liangyue and Tong, Hanghang and Cao, Nan and Ehrlich, Kate and Lin, Yu-Ru and Buchler, Norbou, "Enhancing team composition in professional networks: Problem definitions and fast solutions," *IEEE transactions on knowledge and data engineering*, vol. 29, no. 3, pp. 613–626, 2016.
- [209] Z. Li, X. Pi, M. Wu, and H. Tong, "Reform: Fast and adaptive solution for subteam replacement," in *2021 IEEE International Conference on Big Data (Big Data)*. IEEE, 2021, pp. 350–358.
- [210] C. Hu, Q. Zhou, and H. Tong, "Genius: A novel solution for subteam replacement with clustering-based graph neural network," *arXiv preprint arXiv:2211.04100*, 2022.
- [211] L. Zhao, Y. Yao, G. Guo, H. Tong, F. Xu, and J. Lu, "Team expansion in collaborative environments," in *Pacific-Asia Conference on Knowledge Discovery and Data Mining*. Springer, 2018, pp. 713–725.
- [212] Q. Zhou, L. Li, and H. Tong, "Towards real time team optimization," in *2019 IEEE International Conference on Big Data (Big Data)*. IEEE, 2019, pp. 1008–1017.
- [213] H. Zhao, C. Zhao, X. Zhang, N. Liu, H. Zhu, Q. Liu, and H. Xiong, "An ensemble learning approach with gradient resampling for class-imbalance problems," *INFORMS Journal on Computing*, vol. 35, no. 4, pp. 747–763, 2023.
- [214] K. J. Lauver and A. Kristof-Brown, "Distinguishing between employees' perceptions of person-job and person-organization fit," *Journal of vocational behavior*, vol. 59, no. 3, pp. 454–470, 2001.
- [215] M. Artar, Y. S. Balcioğlu, and O. Erdil, "Improving the quality of hires via the use of machine learning and an expansion of the person-environment fit theory," *Management Decision*, 2024.
- [216] J. Zhu and C. Hudelot, "Towards job-transition-tag graph for a better job title representation learning," *arXiv preprint arXiv:2206.02782*, 2022.
- [217] R. Zbib, L. A. Lacasa, F. Retyk, R. Poves, J. Aizpuru, H. Fabregat, V. Simkus, and E. García-Casademont, "Learning job titles similarity from noisy skill labels," *arXiv preprint arXiv:2207.00494*, 2022.
- [218] L. Malandri, F. Mercurio, M. Mezzanzanica, and N. Nobani, "Meet-Im: A method for embeddings evaluation for taxonomic data in the labour market," *Computers in Industry*, vol. 124, p. 103341, 2021.
- [219] R. Zha, C. Qin, L. Zhang, D. Shen, T. Xu, H. Zhu, and E. Chen, "Career mobility analysis with uncertainty-aware graph autoencoders: A job title transition perspective," *IEEE Transactions on Computational Social Systems*, 2023.
- [220] M. Yamashita, J. T. Shen, T. Tran, H. Ekhtiari, and D. Lee, "James: Normalizing job titles with multi-aspect graph embeddings and reasoning," in *2023 IEEE 10th International Conference on Data Science and Advanced Analytics (DSAA)*. IEEE, 2023, pp. 1–10.
- [221] C. O. Porter, D. E. Cordon, and A. E. Barber, "The dynamics of salary negotiations: Effects on applicants' justice perceptions and recruitment decisions," *International Journal of Conflict Management*, 2004.
- [222] Y. T. Matbouli and S. M. Alghamdi, "Statistical machine learning regression models for salary prediction featuring economy wide activities and occupations," *Information*, vol. 13, no. 10, p. 495, 2022.
- [223] Q. Meng, K. Xiao, D. Shen, H. Zhu, and H. Xiong, "Fine-grained job salary benchmarking with a nonparametric dirichlet process-based latent factor model," *INFORMS Journal on Computing*, 2022.
- [224] C.-C. Hung and E.-P. Lim, "On aggregating salaries of occupations from job post and review data," *IEEE Access*, vol. 9, pp. 43 422–43 433, 2021.
- [225] D. J. Jackson, S. C. Carr, M. Edwards, K. Thorn, N. Allfree, J. Hooks, and K. Inkson, "Exploring the dynamics of new zealand's talent flow," *New Zealand Journal of Psychology*, vol. 34, no. 2, 2005.
- [226] B. Hershbein, C. Macaluso, and C. Yeh, "Concentration in us local labor markets: evidence from vacancy and employment data," Working paper, Tech. Rep., 2018.
- [227] B. Hershbein and L. B. Kahn, "Do recessions accelerate routine-biased technological change? evidence from vacancy postings," *American Economic Review*, vol. 108, no. 7, pp. 1737–72, 2018.
- [228] A. Moniz and F. d. Jong, "Sentiment analysis and the impact of employee satisfaction on firm earnings," in *European conference on information retrieval*. Springer, 2014, pp. 519–527.
- [229] L. Zhang, T. Xu, H. Zhu, C. Qin, Q. Meng, H. Xiong, and E. Chen, "Large-scale talent flow embedding for company competitive analysis," in *Proceedings of The Web Conference 2020*, 2020, pp. 2354–2364.
- [230] L. Zhang, H. Zhu, T. Xu, C. Zhu, C. Qin, H. Xiong, and E. Chen, "Large-scale talent flow forecast with dynamic latent factor model?" in *The World Wide Web Conference*, 2019, pp. 2312–2322.
- [231] B. Liu, Z. Jia, L. Zhao, and W. Kong, "Talent Flow Model Based on Graph Attention Network," in *2023 4th International Conference on Big Data & Artificial Intelligence & Software Engineering (ICBASE)*. Nanjing, China: IEEE, Aug. 2023, pp. 115–121. [Online]. Available: <https://ieeexplore.ieee.org/document/10303067/>
- [232] Y. Cheng, Y. Xie, Z. Chen, A. Agrawal, A. Choudhary, and S. Guo, "Jobminer: A real-time system for mining job-related patterns from social media," in *Proceedings of the 19th ACM SIGKDD international conference on Knowledge discovery and data mining*, 2013, pp. 1450–1453.
- [233] Y. Cheng, "Mining and understanding professional social networks: Challenges and solutions," Ph.D. dissertation, Northwestern University, 2015.
- [234] R. J. Oentaryo, X. J. S. Ashok, E.-P. Lim, and P. K. Prasetyo, "On analyzing job hop behavior and talent flow networks," in *2017 IEEE International Conference on Data Mining Workshops (ICDMW)*. IEEE, 2017, pp. 207–214.
- [235] R. J. Oentaryo, E.-P. Lim, X. J. S. Ashok, P. K. Prasetyo, K. H. Ong, and Z. Q. Lau, "Talent flow analytics in online professional network," *Data Science and Engineering*, vol. 3, no. 3, pp. 199–220, 2018.
- [236] H. Xu, Z. Yu, J. Yang, H. Xiong, and H. Zhu, "Talent circle detection in job transition networks," in *Proceedings of the 22nd ACM SIGKDD International Conference on Knowledge Discovery and Data Mining*, 2016, pp. 655–664.
- [237] P. G. Lovaglio, M. Mezzanzanica, and E. Colombo, "Comparing time series characteristics of official and web job vacancy data," *Quality & Quantity*,



- vol. 54, no. 1, pp. 85–98, 2020.
- [238] I. Karakatsanis, W. AlKhader, F. MacCrory, A. Alibasic, M. A. Omar, Z. Aung, and W. L. Woon, “Data mining approach to monitoring the requirements of the job market: A case study,” *Information Systems*, vol. 65, pp. 1–6, 2017.
- [239] Z. Guo, H. Liu, L. Zhang, Q. Zhang, H. Zhu, and H. Xiong, “Talent Demand-Supply Joint Prediction with Dynamic Heterogeneous Graph Enhanced Meta-Learning,” in *Proceedings of the 28th ACM SIGKDD Conference on Knowledge Discovery and Data Mining*. Washington DC USA: ACM, Aug. 2022. [Online]. Available: <https://dl.acm.org/doi/10.1145/3534678.3539139>
- [240] E. Colombo, F. Mercorio, and M. Mezzananza, “Applying machine learning tools on web vacancies for labour market and skill analysis,” *Terminator or the Jetsons? The Economics and Policy Implications of Artificial Intelligence*, 2018.
- [241] T. M. Akhriza, L. D. Adistia *et al.*, “Constructing recommendation about skills combinations frequently sought in it industries based on apriori algorithm,” in *Mathematics, Informatics, Science, and Education International Conference (MISEIC 2019)*. Atlantis Press, 2019, pp. 24–28.
- [242] F. Patacsil and M. Acosta, “Analyzing the relationship between information technology jobs advertised on-line and skills requirements using association rules,” *Bulletin of Electrical Engineering and Informatics*, vol. 10, no. 5, pp. 2771–2779, 2021.
- [243] I. A. Wowczko, “Skills and vacancy analysis with data mining techniques,” in *Informatics*, vol. 2, no. 4. Multidisciplinary Digital Publishing Institute, 2015, pp. 31–49.
- [244] X. Wu, T. Xu, H. Zhu, L. Zhang, E. Chen, and H. Xiong, “Trend-aware tensor factorization for job skill demand analysis,” in *IJCAI*, 2019, pp. 3891–3897.
- [245] L. Liu, W. Zhang, J. Liu, W. Shi, and Y. Huang, “Learning multi-graph neural network for data-driven job skill prediction,” in *2021 International Joint Conference on Neural Networks (IJCNN)*. IEEE, 2021, pp. 1–8.
- [246] B. Walek and O. Pektor, “Data mining of job requirements in online job advertisements using machine learning and sdca logistic regression,” *Mathematics*, vol. 9, no. 19, p. 2475, 2021.
- [247] F. Leon, M. Gavrilescu, S.-A. Floria, and A. A. Minea, “Hierarchical classification of transversal skills in job advertisements based on sentence embeddings,” *Information*, vol. 15, no. 3, p. 151, 2024.
- [248] J. Mahdaviomghaddam, N. Krishnaswamy, and E. Bagheri, “On the congruence between online social content and future it skill demand,” *Proceedings of the ACM on Human-Computer Interaction*, vol. 5, no. CSCW2, pp. 1–27, 2021.
- [249] J. Mahdaviomghaddam, A. Bahuguna, and E. Bagheri, “Exploring the utility of social content for understanding future in-demand skills,” *Proceedings of the ACM on Human-Computer Interaction*, vol. 6, no. CSCW2, pp. 1–35, 2022.
- [250] M. M. G. de Macedo, W. Clarke, E. Lucherini, T. Baldwin, D. Q. Neto, R. de Paula, and S. Das, “Practical Skills Demand Forecasting via Representation Learning of Temporal Dynamics,” in *Proceedings of the 2022 AAAI/ACM Conference on AI, Ethics, and Society*, Jul. 2022, pp. 285–294.
- [251] V. Wolf, F. Neubürger, and R. Lanwehr, “Generating synthetic data for better prediction modeling in skill demand forecasting,” in *2023 IEEE World Conference on Applied Intelligence and Computing (AIC)*. IEEE, 2023, pp. 313–318.
- [252] W. Chao, Z. Qiu, L. Wu, Z. Guo, Z. Zheng, H. Zhu, and H. Liu, “A Cross-View Hierarchical Graph Learning Hypernetwork for Skill Demand-Supply Joint Prediction,” Jan. 2024.
- [253] H. Rahman, S. Thirumuruganathan, S. B. Roy, S. Amer-Yahia, and G. Das, “Worker skill estimation in team-based tasks,” *Proceedings of the VLDB Endowment*, vol. 8, no. 11, pp. 1142–1153, Jul. 2015.
- [254] F. Stephany and O. Teutloff, “What is the price of a skill? The value of complementarity,” *Research Policy*, vol. 53, no. 1, p. 104898, Jan. 2024.
- [255] Z. Yuan, H. Liu, R. Hu, D. Zhang, and H. Xiong, “Self-Supervised Prototype Representation Learning for Event-Based Corporate Profiling,” *Proceedings of the AAAI Conference on Artificial Intelligence*, vol. 35, no. 5, pp. 4644–4652, May 2021.
- [256] A. Bose and N. Khatoun, “Sentiment analysis of It Companies- Features and Feelings Profiling, as well as Data Mining for Employee Input,” Dec. 2022.
- [257] I. Savin, K. Chukavina, and A. Pushkarev, “Topic-based classification and identification of global trends for startup companies,” *Small Business Economics*, vol. 60, no. 2, pp. 659–689, Feb. 2023.
- [258] B. K. Chae and E. O. Park, “Corporate social responsibility (csr): A survey of topics and trends using twitter data and topic modeling,” *Sustainability*, vol. 10, no. 7, p. 2231, 2018.
- [259] R. Mazza, E. Zavarrone, M. Olivieri, and D. Corsaro, “A text mining approach for CSR communication: an explorative analysis of energy firms on Twitter in the post-pandemic era,” *Italian Journal of Marketing*, vol. 2022, no. 3, pp. 317–340, Sep. 2022.
- [260] K. Pilgrim, J. Koss, and S. Bohnet-Joschko, *CSR Communication on Twitter - A Scoping Review on Social Media Mining and Analytic Methods*, Jan. 2023.
- [261] S. Thakur, A. K. Kar, and N. Sharma, “Impact of Corporate Social Responsibility Orientation of CEOs on Online Reputation-Insights from Text Mining,” in *IoT, Big Data and AI for Improving Quality of Everyday Life: Present and Future Challenges: IOT, Data Science and Artificial Intelligence Technologies*. Cham: Springer International Publishing, 2023, pp. 117–138.
- [262] X. C. Shi and Z. Chen, “Listening to your employees: analyzing opinions from online reviews of hotel companies,” *International Journal of Contemporary Hospitality Management*, vol. 33, no. 6, pp. 2091–2116, Jan. 2021.
- [263] A. Ganga, “Employees Satisfaction in Different Industries: An Exploratory Review of the Literature,” *International Journal of Economics and Management Systems*, vol. 07, Jul. 2022.
- [264] B. Gaye, D. Zhang, and A. Wulamu, “Sentiment classification for employees reviews using regression vector- stochastic gradient descent classifier (RV-SGDC),” *PeerJ Computer Science*, vol. 7, p. e712, Sep. 2021.
- [265] M. S. Rehan, F. Rustam, S. Ullah, S. Hussain, A. Mehmood, and G. S. Choi, “Employees reviews classification and evaluation (ERCE) model using supervised machine learning approaches,” *Journal of Ambient Intelligence and Humanized Computing*, vol. 13, no. 6, pp. 3119–3136, Jun. 2022, 11 citations (Crossref) [2024-04-28].
- [266] N. Mouli, P. Das, M. B. Muquith, A. Biswas, M. D. Kabir Niloy, M. Faisal Ahmed, and D. Z. Karim, “Unveiling Employee Job Satisfaction: Harnessing Deep Learning for Sentiment Analysis,” in *2023 26th International Conference on Computer and Information Technology (ICIT)*. Cox’s Bazar, Bangladesh: IEEE, Dec. 2023, pp. 1–6.
- [267] Xu, Huang and Yu, Zhiwen and Yang, Jingyuan and Xiong, Hui and Zhu, Hengshu, “Dynamic talent flow analysis with deep sequence prediction modeling,” *IEEE Transactions on Knowledge and Data Engineering*, vol. 31, no. 10, pp. 1926–1939, 2018.
- [268] H. Zhu, Y. Sun, W. Zhao, F. Zhuang, B. Wang, and H. Xiong, “Rapid learning of earthquake felt area and intensity distribution with real-time search engine queries,” *Scientific reports*, vol. 10, no. 1, p. 5437, 2020.
- [269] L. Li, T. Lappas, and R. Liu, “Measuring employer attractiveness in diverse talent markets,” *Decision Support Systems*, vol. 177, Feb. 2024. [Online]. Available: <https://linkinghub.elsevier.com/retrieve/pii/S0167923623001549>
- [270] S. Marrara, G. Pasi, M. Viviani, M. Cesarini, F. Mercorio, M. Mezzananza, and M. Pappagallo, “A language modelling approach for discovering novel labour market occupations from the web,” in *Proceedings of the International Conference on Web Intelligence*, 2017, pp. 1026–1034.
- [271] S. H. Azzahra, I. Nurma Yulita, and A. Hidayat, “Text categorization of job vacancy using recurrent neural network method,” in *2021 International Conference on Artificial Intelligence and Big Data Analytics*. Bandung, Indonesia: IEEE, Oct. 2021.
- [272] J. Mahdaviomghaddam, “The Utility of Social Media in Understanding the Future of Work,” in *Companion Publication of the 2022 Conference on Computer Supported Cooperative Work and Social Computing*. Virtual Event Taiwan: ACM, Nov. 2022. [Online]. Available: <https://dl.acm.org/doi/10.1145/3500868.3561397>
- [273] T. Ambler and S. Barrow, “The employer brand,” *Journal of brand management*, vol. 4, no. 3, pp. 185–206, 1996.
- [274] C. N. Arasanmi and A. Krishna, “Employer branding: perceived organisational support and employee retention—the mediating role of organisational commitment,” *Industrial and Commercial Training*, 2019.
- [275] M. Fatma, Z. Rahman, and I. Khan, “Building company reputation and brand equity through csr: the mediating role of trust,” *International Journal of Bank Marketing*, 2015.
- [276] I. Reis, M. J. Sousa, and A. Dionísio, “Employer Branding as a Talent Management Tool: A Systematic Literature Revision,” *Sustainability*, vol. 13, no. 19, p. 10698, Jan. 2021.
- [277] J. O. Krugmann and J. Hartmann, “Sentiment Analysis in the Age of Generative AI,” *Customer Needs and Solutions*, vol. 11, no. 1, p. 3, Dec. 2024.
- [278] S. Kiritchenko and S. M. Mohammad, “Examining gender and race bias in two hundred sentiment analysis systems,” *arXiv preprint arXiv:1805.04508*, 2018.
- [279] A. Koutsoumpis, S. Ghassemi, J. K. Oostrom, D. Holtrop, W. Van Breda, T. Zhang, and R. E. de Vries, “Beyond traditional interviews: Psychometric analysis of asynchronous video interviews for personality and interview performance evaluation using machine learning,” *Computers in Human Behavior*, vol. 154, p. 108128, 2024.
- [280] D. Lahat, T. Adali, and C. Jutten, “Multimodal data fusion: an overview of methods, challenges, and prospects,” *Proceedings of the IEEE*, vol. 103, no. 9, pp. 1449–1477, 2015.
- [281] T. Baltrušaitis, C. Ahuja, and L.-P. Morency, “Multimodal machine learning: A survey and taxonomy,” *IEEE transactions on pattern analysis and machine intelligence*, vol. 41, no. 2, pp. 423–443, 2018.
- [282] K. M. Wiig, “Knowledge management: an introduction and perspective,” *Journal of knowledge Management*, 1997.
- [283] S. Ji, S. Pan, E. Cambria, P. Marttinen, and S. Y. Philip, “A survey on knowledge graphs: Representation, acquisition, and applications,” *IEEE Transactions on Neural Networks and Learning Systems*, 2021.
- [284] C. Wang, H. Zhu, P. Wang, C. Zhu, X. Zhang, E. Chen, and H. Xiong, “Personalized and explainable employee training course recommendations: A bayesian variational approach,” *ACM Transactions on Information Systems (TOIS)*, vol. 40, no. 4, pp. 1–32, 2021.
- [285] J. Harrigan, A. Reshef, and F. Toubal, “The march of the techies: Job polarization within and between firms,” *Research Policy*, vol. 50, no. 7, p. 104008, 2021.
- [286] T. Babina, A. Fedyk, A. He, and J. Hodson, “Artificial intelligence, firm growth, and product innovation,” *Journal of Financial Economics*, vol. 151, p. 103745, 2024.
- [287] J. Kim, A. Rai, and Y.-K. Lin, “Ai labor markets: Toward a dynamic skills-based approach to measurement,” in *(International Conference on Information Systems 2023)*, 2023.
- [288] B. Groyberg, J. Lee, J. Price, and J. Y.-J. Cheng, “The

- leader's guide to corporate culture," <https://hbr.org/2018/01/the-leaders-guide-to-corporate-culture>, 2018.
- [289] A. Lee, I. Inceoglu, O. Hauser, and M. Greene, "Determining causal relationships in leadership research using machine learning: The powerful synergy of experiments and data science," *The Leadership Quarterly*, p. 101426, 2020.
- [290] W. Ahmad, M. Akhtaruzamman, U. Zahra, C. Ohri, and B. Ramakrishnan, "Investigation on the impact of leadership styles using data mining techniques," *Leadership*, 2018.
- [291] J. Dastin, "Amazon scraps secret ai recruiting tool that showed bias against women," <https://www.reuters.com/article/us-amazon-com-jobs-automation-insight-idUSKCN1MK08G>, 2018.
- [292] S. Yan, D. Huang, and M. Soleymani, "Mitigating biases in multimodal personality assessment," in *Proceedings of the 2020 International Conference on Multimodal Interaction*, 2020, pp. 361–369.
- [293] L. Wu, Z. Zheng, Z. Qiu, H. Wang, H. Gu, T. Shen, C. Qin, C. Zhu, H. Zhu, Q. Liu et al., "A survey on large language models for recommendation," *arXiv preprint arXiv:2305.19860*, 2023.
- [294] S. B. Zinjad, A. Bhattacharjee, A. Bhilegaonkar, and H. Liu, "Resumeflow: An llm-facilitated pipeline for personalized resume generation and refinement," *arXiv preprint arXiv:2402.06221*, 2024.
- [295] T. Guo, X. Chen, Y. Wang, R. Chang, S. Pei, N. V. Chawla, O. Wiest, and X. Zhang, "Large language model based multi-agents: A survey of progress and challenges," *arXiv preprint arXiv:2402.01680*, 2024.
- [296] E. W. Ellinger, R. W. Gregory, T. Mini, T. Widjaja, and O. Henfridsson, "Skin in the game: The transformational potential of decentralized autonomous organizations," *MIS Quarterly*, 2023.
- [297] Z. Liu, Y. Zhang, P. Li, Y. Liu, and D. Yang, "Dynamic llm-agent network: An llm-agent collaboration framework with agent team optimization," *arXiv preprint arXiv:2310.02170*, 2023.
- [298] C. Xie, C. Chen, F. Jia, Z. Ye, K. Shu, A. Bibi, Z. Hu, P. Torr, B. Ghanem, and G. Li, "Can large language model agents simulate human trust behaviors?" *arXiv preprint arXiv:2402.04559*, 2024.
- [299] S. G. Bouschery, V. Blazevic, and F. T. Piller, "Augmenting human innovation teams with artificial intelligence: Exploring transformer-based language models," *Journal of Product Innovation Management*, vol. 40, no. 2, pp. 139–153, 2023.
- [300] M. R. Hasan, R. K. Ray, and F. R. Chowdhury, "Employee performance prediction: An integrated approach of business analytics and machine learning," *Journal of Business and Management Studies*, vol. 6, no. 1, pp. 215–219, 2024.
- [301] Y.-C. Chang, C.-H. Ku, and D.-D. Le Nguyen, "Predicting aspect-based sentiment using deep learning and information visualization: The impact of covid-19 on the airline industry," *Information & Management*, vol. 59, no. 2, p. 103587, 2022.
- [302] A. M. Shah, X. Yan, A. Qayyum, R. A. Naqvi, and S. J. Shah, "Mining topic and sentiment dynamics in physician rating websites during the early wave of the covid-19 pandemic: Machine learning approach," *International Journal of Medical Informatics*, vol. 149, p. 104434, 2021.
- [303] K. D. Strang and Z. Sun, "Erp staff versus ai recruitment with employment real-time big data," *Discover Artificial Intelligence*, vol. 2, no. 1, p. 21, 2022.
- [304] S. Westberg, "Applying a chatbot for assistance in the onboarding process: A process of requirements elicitation and prototype creation," 2019.
- [305] D. Vrontis, M. Christofi, V. Pereira, S. Tarba, A. Makrides, and E. Trichina, "Artificial intelligence, robotics, advanced technologies and human resource management: a systematic review," *The international journal of human resource management*, vol. 33, no. 6, pp. 1237–1266, 2022.
- [306] H. Kroppu-Vehkaperä, H. Haaapasalo, J. Harkonen, and R. Silvola, "Product data management practices in high-tech companies," *Industrial Management & Data Systems*, vol. 109, no. 6, pp. 758–774, Jun. 2009.
- [307] E. Shehab, M. Sharp, L. Supramaniam, and T. Spedding, "Enterprise resource planning: An integrative review," *Business Process Management Journal*, vol. 10, no. 4, pp. 359–386, Aug. 2004.
- [308] P. Frow and A. Payne, "Customer Relationship Management: A Strategic Perspective," *Journal of business market management*, vol. 3, no. 1, pp. 7–27, Feb. 2009.
- [309] A. N. Mukherjee, S. Bhattacharyya, and R. Bera, "Role of information technology in human resource management of sme: A study on the use of applicant tracking system," *IBMRD's Journal of Management & Research*, pp. 1–22, 2014.
- [310] Q. Kong, Y. Cai, and Q. Zhu, "The case study for the basic information service of job post resource based on web mining," in *2012 International Conference on Computer Science and Service System*. IEEE, 2012, pp. 498–501.
- [311] W.-W. Wu, Y.-T. Lee, and G.-H. Tzeng, "Simplifying the manager competency model by using the rough set approach," in *International Workshop on Rough Sets, Fuzzy Sets, Data Mining, and Granular-Soft Computing*. Springer, 2005, pp. 484–494.
- [312] W. Hong and Y. Wang, "Evaluation of highway construction foreman's competency based on support vector machine," in *Journal of Physics: Conference Series*, vol. 1168, no. 3. IOP Publishing, 2019, p. 032106.
- [313] A. Elragal, "Erp and big data: The inept couple," *Procedia Technology*, vol. 16, pp. 242–249, 2014.
- [314] M. Bakaev and T. Avdeenko, "Intelligent information system to support decision-making based on unstructured web data," *ICIC Express Letters*, vol. 9, no. 4, pp. 1017–1023, 2015.
- [315] M. Theobald, H. Bast, D. Majumdar, R. Schenkel, and G. Weikum, "Topx: efficient and versatile top-k query processing for semistructured data," *The VLDB Journal*, vol. 17, pp. 81–115, 2008.
- [316] C. Signore, B. Della Piana, and F. Di Vincenzo, "Digital job searching and recruitment platforms: A semi-systematic literature review," in *International Conference in Methodologies and Intelligent Systems for Technology Enhanced Learning*. Springer, 2023, pp. 313–322.
- [317] C. Zhang and H. Wang, "Resumevis: A visual analytics system to discover semantic information in semi-structured resume data," *ACM Transactions on Intelligent Systems and Technology (TIST)*, vol. 10, no. 1, pp. 1–25, 2018.
- [318] E. Boštjančič and Z. Slana, "The role of talent management comparing medium-sized and large companies—major challenges in attracting and retaining talented employees," *Frontiers in psychology*, vol. 9, p. 396740, 2018.
- [319] W. Cohen and L. Jensen, "A structured wrapper induction system for extracting information from semi-structured documents," in *Proceedings of the Workshop on Adaptive Text Extraction and Mining (IJCAI'01)*. Citeseer, 2001.
- [320] A. De Mauro, M. Greco, M. Grimaldi, and P. Ritala, "Human resources for big data professions: A systematic classification of job roles and required skill sets," *Information Processing & Management*, vol. 54, no. 5, pp. 807–817, 2018.
- [321] S. Vijayarani, M. J. Ilamathi, M. Nithya et al., "Preprocessing techniques for text mining—an overview," *International Journal of Computer Science & Communication Networks*, vol. 5, no. 1, pp. 7–16, 2015.
- [322] B. Balducci and D. Marinova, "Unstructured data in marketing," *Journal of the Academy of Marketing Science*, vol. 46, pp. 557–590, 2018.
- [323] R. Boselli, M. Cesarini, S. Marrara, F. Mercurio, M. Mezzanzanica, G. Pasi, and M. Viviani, "Wolmis: A labor market intelligence system for classifying web job vacancies," *Journal of intelligent information systems*, vol. 51, pp. 477–502, 2018.
- [324] D. C. Corrales, J. C. Corrales, and A. Ledezma, "How to address the data quality issues in regression models: A guided process for data cleaning," *Symmetry*, vol. 10, no. 4, p. 99, 2018.
- [325] Y. Huang, "Study of college human resources data mining based on the som algorithm," in *2009 Asia-Pacific Conference on Information Processing*, vol. 1. IEEE, 2009, pp. 324–327.
- [326] T. Shao, C. Song, J. Zheng, F. Cai, H. Chen et al., "Exploring internal and external interactions for semi-structured multivariate attributes in job-resume matching," *International Journal of Intelligent Systems*, vol. 2023, 2023.
- [327] J. Balaji, M. Sigdel, P. Hoang, M. Liu, and M. Korayem, "Airesume: Automated generation of resume work history," in *KaRS@ CIKM*, 2019, pp. 19–25.
- [328] M. Beresewicz, H. Cherniaev, A. Mantaj, and R. Pater, "Text analysis of job offers for mismatch of educational characteristics to labour market demands," *Quality & Quantity*, vol. 58, no. 2, pp. 1799–1825, 2024.
- [329] S. Gaikwad and N. Bogiri, "Effective and efficient xml duplicate detection using levenshtein distance algorithm,"
- [330] Z. Chuang, W. Ming, L. C. Guang, X. Bo, and L. Zhi-qing, "Resume parser: Semi-structured chinese document analysis," in *2009 WRI world congress on computer science and information engineering*, vol. 5. IEEE, 2009, pp. 12–16.
- [331] S. Pawar, R. Srivastava, and G. K. Palshikar, "Automatic gazette creation for named entity recognition and application to resume processing," in *Proceedings of the 5th ACM COMPUTE Conference: Intelligent & scalable system technologies*, 2012, pp. 1–7.
- [332] J. Luo, Y. Liu, and M. Hou, "A novel chinese resume named entity recognition model based on lexical enhancement," in *Proceedings of the 2022 11th International Conference on Computing and Pattern Recognition*, 2022, pp. 341–346.
- [333] J. Zhenhong, P. Lingxi, and S. Lei, "Person-job fit model based on sentence-level representation and theme-word graph," in *2021 IEEE 5th Advanced Information Technology, Electronic and Automation Control Conference (IAEAC)*, vol. 5. IEEE, 2021, pp. 1902–1909.
- [334] R. Yan, R. Le, Y. Song, T. Zhang, X. Zhang, and D. Zhao, "Interview choice reveals your preference on the market: To improve job-resume matching through profiling memories," in *Proceedings of the 25th ACM SIGKDD International Conference on Knowledge Discovery & Data Mining*, 2019, pp. 914–922.
- [335] Z. Guan, J.-Q. Yang, Y. Yang, H. Zhu, W. Li, and H. Xiong, "Jobformer: Skill-aware job recommendation with semantic-enhanced transformer," *arXiv preprint arXiv:2404.04313*, 2024.
- [336] Z. Gong, Y. Song, T. Zhang, J.-R. Wen, D. Zhao, and R. Yan, "Your career path matters in person-job fit," in *Proceedings of the AAAI Conference on Artificial Intelligence*, vol. 38, no. 8, 2024, pp. 8427–8435.
- [337] H. Chen, L. Du, Y. Lu, Q. Fu, X. Chen, S. Han, Y. Kang, G. Lu, and Z. Li, "Professional network matters: Connections empower person-job fit," in *Proceedings of the 17th ACM International Conference on Web Search and Data Mining*, 2024, pp. 96–105.
- [338] P. Ghosh and V. Sadaphal, "Jobrecogpt—explainable job recommendations using llms," *arXiv preprint arXiv:2309.11805*, 2023.
- [339] L. Wu, Z. Qiu, Z. Zheng, H. Zhu, and E. Chen, "Exploring large language model for graph data understanding in online job recommendations," in *Proceedings of the AAAI Conference on Artificial Intelligence*, vol. 38, no. 8, 2024, pp. 9178–9186.
- [340] E. Faliagka, A. Tsakalidis, and G. Tzimas, "An integrated e-recruitment system for automated personality mining and applicant ranking," *Internet research*, 2012.
- [341] A. Giri, A. Ravikumar, S. Mote, and R. Bharadwaj, "Vritthi-a theoretical framework for it recruitment based on machine learning techniques ap-



- plied over twitter, linkedin, spoj and github profiles," in *2016 International Conference on Data Mining and Advanced Computing (SAPIENCE)*. IEEE, 2016, pp. 1–7.
- [342] V. M. Menon and H. Rahulnath, "A novel approach to evaluate and rank candidates in a recruitment process by estimating emotional intelligence through social media data," in *2016 International Conference on Next Generation Intelligent Systems (ICNGIS)*. IEEE, 2016, pp. 1–6.
- [343] F. Borisyuk, L. Zhang, and K. Kenthapadi, "Lijar: A system for job application redistribution towards efficient career marketplace," in *Proceedings of the 23rd ACM SIGKDD International Conference on Knowledge Discovery and Data Mining*, 2017, pp. 1397–1406.
- [344] Naim, Iftekhar and Tanveer, Md Iftekhar and Gildea, Daniel and Hoque, Mohammed Ehsan, "Automated analysis and prediction of job interview performance," *IEEE Transactions on Affective Computing*, vol. 9, no. 2, pp. 191–204, 2016.
- [345] L. Hemamou, A. Guillon, J.-C. Martin, and C. Clavel, "Multimodal hierarchical attention neural network: Looking for candidates behaviour which impact recruiter's decision," *IEEE Transactions on Affective Computing*, vol. 14, no. 2, pp. 969–985, 2021.
- [346] R. Verrap, E. Nirjhar, A. Nenikova, and T. Chaspari, "'am i answering my job interview questions right?': A nlp approach to predict degree of explanation in job interview responses," in *Proceedings of the Second Workshop on NLP for Positive Impact (NLP4PI)*, 2022, pp. 122–129.
- [347] D. S. Sisodia, S. Vishwakarma, and A. Pujahari, "Evaluation of machine learning models for employee churn prediction," in *2017 international conference on inventive computing and informatics (icici)*. IEEE, 2017, pp. 1016–1020.
- [348] P. Ajit, "Prediction of employee turnover in organizations using machine learning algorithms," *algorithms*, vol. 4, no. 5, p. C5, 2016.
- [349] P. Guo, K. Xiao, H. Zhu, and Q. Meng, "Preference-constrained career path optimization: An exploration space-aware stochastic model," in *2023 IEEE International Conference on Data Mining (ICDM)*. IEEE, 2023, pp. 120–129.
- [350] S. Avlonitis, D. Lavi, M. Mansoury, and D. Graus, "Career path recommendations for long-term income maximization: A reinforcement learning approach," *arXiv preprint arXiv:2309.05391*, 2023.
- [351] S. Krishnan, D. Haas, M. J. Franklin, and E. Wu, "Towards reliable interactive data cleaning: A user survey and recommendations," in *Proceedings of the Workshop on Human-in-the-Loop Data Analytics*, 2016, pp. 1–5.
- [352] H. Liu and H. Motoda, *Feature extraction, construction and selection: A data mining perspective*. Springer Science & Business Media, 1998, vol. 453.
- [353] S. Guo, F. Alamudun, and T. Hammond, "Résumatcher: A personalized résumé-job matching system," *Expert Systems with Applications*, vol. 60, pp. 169–182, 2016.
- [354] R. Muthyala, S. Wood, Y. Jin, Y. Qin, H. Gao, and A. Rai, "Data-driven job search engine using skills and company attribute filters," in *2017 IEEE International Conference on Data Mining Workshops (ICDMW)*. IEEE, 2017, pp. 199–206.
- [355] A. Wakchaure, R. Eaglin, and B. Motlagh, "A technique for the quantitative measure of data cleanliness," in *2008 IEEE Conference on Cybernetics and Intelligent Systems*. IEEE, 2008, pp. 1258–1263.
- [356] A. Magron, A. Dai, M. Zhang, S. Montariol, and A. Bosselut, "Jobskape: A framework for generating synthetic job postings to enhance skill matching," *arXiv preprint arXiv:2402.03242*, 2024.
- [357] P. Skondras, P. Zervas, and G. Tzimas, "Generating synthetic resume data with large language models for enhanced job description classification," *Future Internet*, vol. 15, no. 11, p. 363, 2023.
- [358] M. Friedrich, A. Köhn, G. Wiedemann, and C. Biemann, "Adversarial learning of privacy-preserving text representations for de-identification of medical records," in *Proceedings of the 57th Annual Meeting of the Association for Computational Linguistics*, A. Korhonen, D. Traum, and L. Marquez, Eds. Florence, Italy: Association for Computational Linguistics, Jul. 2019, pp. 5829–5839. [Online]. Available: <https://aclanthology.org/P19-1584>
- [359] J. Trienes, D. Trieschnigg, C. Seifert, and D. Hiemstra, "Comparing rule-based, feature-based and deep neural methods for de-identification of dutch medical records," *arXiv preprint arXiv:2001.05714*, 2020.
- [360] R. Chevrier, V. Foufi, C. Gaudet-Blavignac, A. Robert, and C. Lovis, "Use and understanding of anonymization and de-identification in the biomedical literature: scoping review," *Journal of medical Internet research*, vol. 21, no. 5, p. e13484, 2019.
- [361] K. N. Jensen, M. Zhang, and B. Plank, "De-identification of privacy-related entities in job postings," in *Proceedings of the 23rd Nordic Conference on Computational Linguistics (NoDaLiDa)*, S. Dobnik and L. Øvrelid, Eds. Reykjavik, Iceland (Online): Linköping University Electronic Press, Sweden, May 31–2 Jun. 2021, pp. 210–221. [Online]. Available: <https://aclanthology.org/2021.nodalida-main.21>
- [362] Z. Dong, X. Huang, G. Yuan, H. Zhu, and H. Xiong, "Butterfly-core community search over labeled graphs," *arXiv preprint arXiv:2105.08628*, 2021.
- [363] X. Wang, X. Zhang, Y. Cheng, F. Tian, K. Chen, and P. O. de Pablos, "Artificial intelligence-enabled knowledge management," *The Routledge Companion to Knowledge Management*, pp. 153–168, 2022.
- [364] P. Huang and Z. Zhang, "Participation in open knowledge communities and job-hopping," *MIS Quarterly*, vol. 40, no. 3, pp. 785–806, 2016.
- [365] Y. Zhang and Q. Yang, "A survey on multi-task learning," *IEEE Transactions on Knowledge and Data Engineering*, 2021.
- [366] C. Zhang, D. Song, C. Huang, A. Swami, and N. V. Chawla, "Heterogeneous graph neural network," in *Proceedings of the 25th ACM SIGKDD International Conference on Knowledge Discovery & Data Mining*, 2019, pp. 793–803.
- [367] M. Goos, E. Rademakers, and R. Roettger, "Routine-biased technical change: Individual-level evidence from a plant closure," *Research Policy*, vol. 50, no. 7, p. 104002, 2021.
- [368] K. Li, X. Liu, F. Mai, and T. Zhang, "The role of corporate culture in bad times: Evidence from the covid-19 pandemic," *Journal of Financial and Quantitative Analysis*, vol. 56, no. 7, pp. 2545–2583, 2021.
- [369] M. K. Lee, "Understanding perception of algorithmic decisions: Fairness, trust, and emotion in response to algorithmic management," *Big Data & Society*, vol. 5, no. 1, p. 2053951718756684, 2018.
- [370] M. Bogen, "All the ways hiring algorithms can introduce bias," *Harvard Business Review*, vol. 6, p. 2019, 2019.
- [371] B. d'Alessandro, C. O'Neil, and T. LaGatta, "Conscientious classification: A data scientist's guide to discrimination-aware classification," *Big data*, vol. 5, no. 2, pp. 120–134, 2017.
- [372] M. De-Arteaga, A. Romanov, H. Wallach, J. Chayes, C. Borgs, A. Chouldechova, S. Geyik, K. Kenthapadi, and A. T. Kalai, "Bias in bios: A case study of semantic representation bias in a high-stakes setting," in *proceedings of the Conference on Fairness, Accountability, and Transparency*, 2019, pp. 120–128.
- [373] A. Morales, J. Fierrez, R. Vera-Rodriguez, and R. Tolosana, "Sensitivenets: Learning agnostic representations with application to face images," *IEEE Transactions on Pattern Analysis and Machine Intelligence*, vol. 43, no. 6, pp. 2158–2164, 2020.
- [374] R. K. Bellamy, K. Dey, M. Hind, S. C. Hoffman, S. Houde, K. Kannan, P. Lohia, J. Martino, S. Mehta, A. Mojsilovic et al., "Ai fairness 360: An extensible toolkit for detecting, understanding, and mitigating unwanted algorithmic bias," *arXiv preprint arXiv:1810.01943*, 2018.
- [375] J. A. Adebayo et al., "Fairml: Toolbox for diagnosing bias in predictive modeling," Ph.D. dissertation, Massachusetts Institute of Technology, 2016.
- [376] N. Bantilan, "Themis-ml: A fairness-aware machine learning interface for end-to-end discrimination discovery and mitigation," *Journal of Technology in Human Services*, vol. 36, no. 1, pp. 15–30, 2018.
- [377] D. F. Mujtaba and N. R. Mahapatra, "Ethical considerations in ai-based recruitment," in *2019 IEEE International Symposium on Technology and Society (ISTAS)*. IEEE, 2019, pp. 1–7.
- [378] G. Mann and C. O'Neil, "Hiring algorithms are not neutral," <https://hbr.org/2016/12/hiring-algorithms-are-not-neutral>, 2016.
- [379] A. L. Hunkenschroer and C. Luetge, "Ethics of ai-enabled recruiting and selection: A review and research agenda," *Journal of Business Ethics*, pp. 1–31, 2022.
- [380] X. Zhang, Y. Zhao, X. Tang, H. Zhu, and H. Xiong, "Developing fairness rules for talent intelligence management system," in *Proceedings of the 53rd Hawaii International Conference on System Sciences*, 2020.
- [381] C. Upadhyay, H. Abu-Rasheed, C. Weber, and M. Fathi, "Explainable job-posting recommendations using knowledge graphs and named entity recognition," in *2021 IEEE International Conference on Systems, Man, and Cybernetics (SMC)*. IEEE, 2021, pp. 3291–3296.
- [382] H. Kaya, F. Gurpinar, and A. Ali Salah, "Multi-modal score fusion and decision trees for explainable automatic job candidate screening from video cvs," in *Proceedings of the IEEE conference on computer vision and pattern recognition workshops*, 2017, pp. 1–9.
- [383] C. Liem, M. Langer, A. Demetriou, A. M. Hiemstra, A. Sukma Wicaksana, M. P. Born, and C. J. König, "Psychology meets machine learning: Interdisciplinary perspectives on algorithmic job candidate screening," *Explainable and interpretable models in computer vision and machine learning*, pp. 197–253, 2018.
- [384] J. Choo and S. Liu, "Visual analytics for explainable deep learning," *IEEE computer graphics and applications*, vol. 38, no. 4, pp. 84–92, 2018.
- [385] G. Alicioglu and B. Sun, "A survey of visual analytics for explainable artificial intelligence methods," *Computers & Graphics*, vol. 102, pp. 502–520, 2022.
- [386] L. Wang, C. Ma, X. Feng, Z. Zhang, H. Yang, J. Zhang, Z. Chen, J. Tang, X. Chen, Y. Lin et al., "A survey on large language model based autonomous agents," *Frontiers of Computer Science*, vol. 18, no. 6, pp. 1–26, 2024.
- [387] N. Ayoobi, S. Shahriar, and A. Mukherjee, "The looming threat of fake and llm-generated linkedin profiles: Challenges and opportunities for detection and prevention," in *Proceedings of the 34th ACM Conference on Hypertext and Social Media*, 2023, pp. 1–10.
- [388] H. Abu-Rasheed, M. H. Abdulsalam, C. Weber, and M. Fathi, "Supporting student decisions on learning recommendations: An llm-based chatbot with knowledge graph contextualization for conversational explainability and mentoring," *arXiv preprint arXiv:2401.08517*, 2024.
- [389] M. A. K. Raiaan, M. S. H. Mukta, K. Fatema, N. M. Fahad, S. Sakib, M. M. J. Mim, J. Ahmad, M. E. Ali, and S. Azam, "A review on large language models: Architectures, applications, taxonomies, open issues and challenges," *IEEE Access*, 2024.
- [390] Z. Yang, A. Liu, Z. Liu, K. Liu, F. Xiong, Y. Wang, Z. Yang, Q. Hu, X. Chen, Z. Zhang et al., "Towards unified alignment between agents, humans, and environment," *arXiv preprint arXiv:2402.07744*, 2024.
- [391] G. Li, H. Hammoud, H. Itani, D. Khizbullin, and B. Ghanem, "Camel: Communicative agents for "mind" exploration of large language model society," *Advances in Neural Information Processing Systems*, vol. 36, 2024.
- [392] A. Pan, E. Jones, M. Jagadeesan, and J. Steinhardt, "Feedback loops with language models drive in-context reward hacking," *arXiv preprint arXiv:2402.06627*, 2024.
- [393] Z. Chu, Y. Wang, F. Zhu, L. Yu, L. Li, and J. Gu, "Professional agents–

- evolving large language models into autonomous experts with human-level competencies," *arXiv preprint arXiv:2402.03628*, 2024.
- [394] S. Wang, H. Yuan, L. M. Ni, and J. Guo, "Quantagent: Seeking holy grail in trading by self-improving large language model," *arXiv preprint arXiv:2402.03755*, 2024.
  - [395] J. Yang, J. Dong, Q. Song, Y. S. Otmakhova, and Z. He, "The impacts of payment policy on performance of human resource market system: Agent-based modeling and simulation of growth-oriented firms," *Systems*, vol. 11, no. 6, p. 298, 2023.
  - [396] W. L. Kuechler and V. Vaishnavi, "So, talk to me: The effect of explicit goals on the comprehension of business process narratives," *Mis Quarterly*, pp. 961–979, 2006.
  - [397] X. Guo, K. Huang, J. Liu, W. Fan, N. Vélez, Q. Wu, H. Wang, T. L. Griffiths, and M. Wang, "Embodied llm agents learn to cooperate in organized teams," *arXiv preprint arXiv:2403.12482*, 2024.
  - [398] A. Susarla, R. Gopal, J. B. Thatcher, and S. Sarker, "The janus effect of generative ai: Charting the path for responsible conduct of scholarly activities in information systems," *Information Systems Research*, vol. 34, no. 2, pp. 399–408, 2023.
  - [399] J. Deng and Y. Lin, "The benefits and challenges of chatgpt: An overview," *Frontiers in Computing and Intelligent Systems*, vol. 2, no. 2, pp. 81–83, 2022.
  - [400] A. Shulner-Tal, T. Kuflik, and D. Kliger, "Fairness, explainability and in-between: understanding the impact of different explanation methods on non-expert users' perceptions of fairness toward an algorithmic system," *Ethics and Information Technology*, vol. 24, no. 1, p. 2, 2022.
  - [401] Y. Wang, Y. Pan, M. Yan, Z. Su, and T. H. Luan, "A survey on chatgpt: Ai-generated contents, challenges, and solutions," *IEEE Open Journal of the Computer Society*, 2023.
  - [402] A. Garlapati, D. R. Krishna, K. Garlapati, and G. Narayanan, "Predicting employees under stress for pre-emptive remediation using machine learning algorithm," in *2020 International Conference on Recent Trends on Electronics, Information, Communication & Technology (RTEICT)*. IEEE, 2020, pp. 315–319.
  - [403] F. Mozaffari, M. Rahimi, H. Yazdani, and B. Sohrabi, "Employee attrition prediction in a pharmaceutical company using both machine learning approach and qualitative data," *Benchmarking: An International Journal*, vol. 30, no. 10, pp. 4140–4173, 2023.
  - [404] S. M. Tharani and S. V. Raj, "Predicting employee turnover intention in it&ites industry using machine learning algorithms," in *2020 Fourth International Conference on I-SMAC (IoT in Social, Mobile, Analytics and Cloud)(I-SMAC)*. IEEE, 2020, pp. 508–513.
  - [405] M. G. Celbiş, P.-h. Wong, K. Kourtiti, and P. Nijkamp, "Impacts of the covid-19 outbreak on older-age cohorts in european labor markets: A machine learning exploration of vulnerable groups," *Regional Science Policy & Practice*, vol. 15, no. 3, pp. 559–585, 2023.
  - [406] A. A. Alaql, F. Alqurashi, and R. Mehmood, "Multi-generational labour markets: data-driven discovery of multi-perspective system parameters using machine learning," *Science Progress*, vol. 106, no. 4, p. 00368504231213788, 2023.
  - [407] A. Mer and A. S. Virdi, "Navigating the paradigm shift in hrm practices through the lens of artificial intelligence: A post-pandemic perspective," *The Adoption and Effect of Artificial Intelligence on Human Resources Management, Part A*, pp. 123–154, 2023.
  - [408] D. Xu and X. Xiao, "Influence of the development of vr technology on enterprise human resource management in the era of artificial intelligence," *IEEE Access*, 2020.
  - [409] M. M. Matonya, "Innovation, artificial intelligence in contingent work-force management," *International Journal of Engineering and Management Sciences*, vol. 5, no. 1, pp. 571–590, 2020.
